# Supplementary material for: Flashy Backdoor: Real-world Environment Backdoor Attack on SNNs with DVS Cameras
Source: arXiv:2411.03022 source file (2024-11-05)
Supplement: Supplementary file 1 [file DVS_Appendix.tex]

SNNs are particularly well-suited for processing high temporal-resolution data. Hence, they are commonly applied to neuromorphic data (see Figure~\ref{fig:neuromorphic}), which presents a time-encoded depiction of the relative luminosity changes in a scene, typically captured by a DVS camera, also known as event-based cameras. DVS cameras are bio-inspired devices that mimic the human retina's asynchronous processing~\cite{Gallego}. These sensors independently detect changes in light intensity at each pixel, producing asynchronous events only when a change is detected. This approach allows for low-latency and high-dynamic-range imaging, making DVS cameras particularly effective in scenarios where traditional frame-based cameras struggle, such as in high-speed motion or challenging lighting conditions~\cite{Gallego}.

\begin{figure}[ht]
    \centering
    \includegraphics[width = \linewidth]{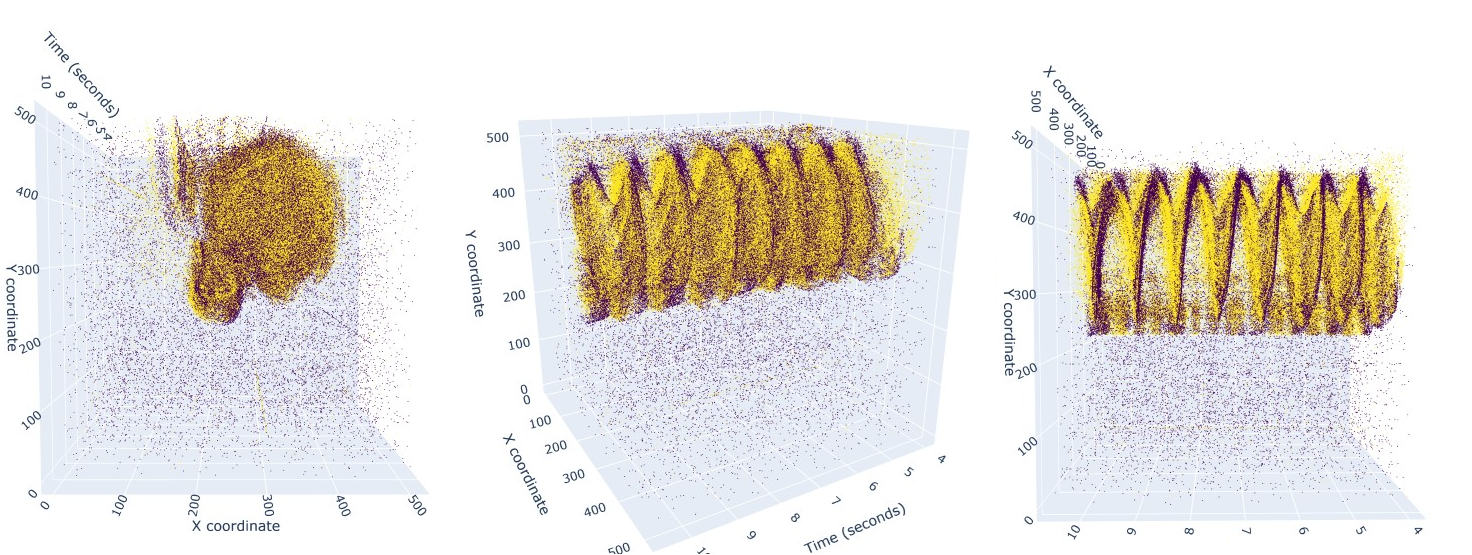}
    \caption{One sample we captured with a DVS camera of a subject moving their left arm in a rotational counter-clockwise motion, depicting both \emph{ON} (yellow) and \emph{OFF} (dark purple) events through a sample of 12 seconds.}
    \label{fig:neuromorphic}
\end{figure}

The pixel operation in a DVS involves three main components~\cite{Lichtsteiner}: a photoreceptor, a differencing circuit, and a comparator. The photoreceptor measures light intensity and converts it into a logarithmic signal. The differencing circuit compares the current intensity to a stored reference value. When the difference exceeds a predefined threshold, the comparator generates an event (see Figure~\ref{fig:DVSwork}). Events are categorized as positive ($ON$) for increases in intensity and negative ($OFF$) for decreases.

\begin{figure}[ht]
    \centering
    \includegraphics[width = 0.75\linewidth]{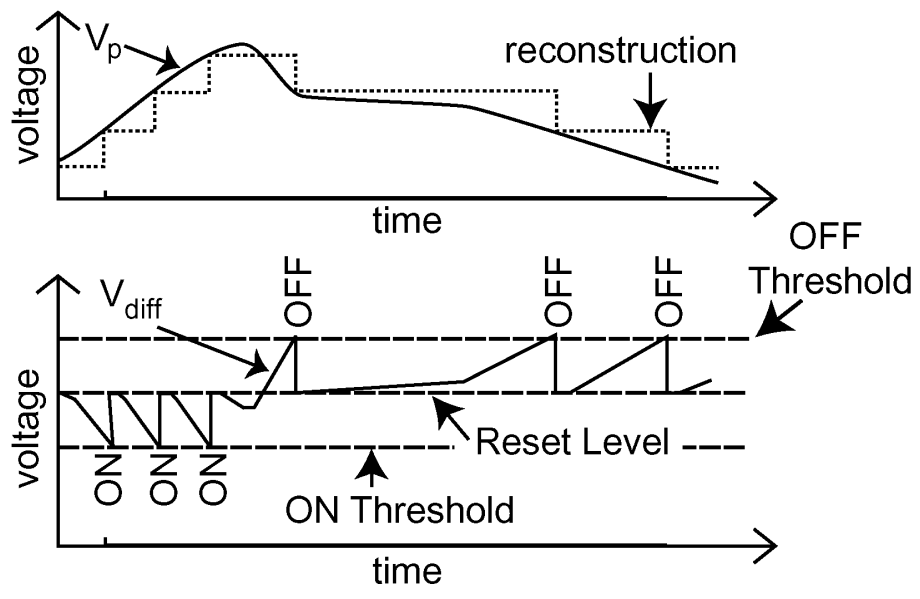}
    \caption{Principle of operation of a DVS as depicted by Lichtsteiner et al.~\cite{Lichtsteiner}.}
    \label{fig:DVSwork}
\end{figure}

Each event recorded by a DVS includes specific data: the $\{X, Y\}$ coordinates of the pixel location, the polarity $p$ indicating whether the change is an increase or decrease in light intensity and a timestamp $T$ that provides the precise time of the event, usually measured in microseconds. This efficient encoding scheme helps to reduce the energy consumption for computation~\cite{eficient}.

Unlike traditional cameras, DVS cameras capture data as a continuous stream of spiking events, dynamically reflecting changes in the observed scene. The primary advantage of such cameras lies in their ability to provide a highly compressed representation of the captured information, resulting in minimal delay and exceptional temporal resolution~\cite{DVS}. Moreover, the event-based nature of DVS data means that it inherently provides a sparse representation of the visual scene~\cite{DL_SNN}, which is beneficial for both storage and computational efficiency. This sparsity is particularly advantageous for SNNs, which compute temporal spikes rather than continuous signals, thus reducing power consumption and enhancing processing speed~\cite{Lichtsteiner}. Additionally, DVS cameras offer high temporal resolution, typically in the microsecond range, enabling the capture of high-speed changes that are not detectable with conventional cameras~\cite{Brandli}.
These capabilities make DVS cameras especially useful in scenarios requiring low-power consumption or high-speed processing, like in real-time applications on robotics~\cite{roboti_pencil} or autonomous driving~\cite{SNN_driving}.
