# Supplementary material for: Flashy Backdoor: Real-world Environment Backdoor Attack on SNNs with DVS Cameras
Source: arXiv:2411.03022 source file (2024-11-05)
Supplement: Supplementary file 2 [file appendixA.tex]

\todo{R:change this appendix}
This section contains the rest of the results obtained from the analysis. \autoref{fig:gestures_graphs} displays all graphs generated from performing the Framed attack on the DVS128-gesture dataset. The graphs show the effect of various trigger sizes and frame lengths across all three temporal positions, considering every possible polarity on the ASR and Clean Accuracy. 
% \todo{?}

As previously noted, there is an inverse relationship between the trigger size and the number of frames required for a successful attack. Additionally, increased trigger size contributes to more stable backdoor training. On the other hand, we observe no significant effect on the clean accuracy of the attacked models with any parameter change on this dataset.
Additionally, polarity $p=0$ performs the worst for both attacks when using small triggers. This was expected, as most of the activations in this dataset are centered in the middle of the frame, containing only noise on the edges. Inserting a small patch with polarity $p=0$  makes it challenging for the model to learn the backdoor behavior, as most of the time, that same region does not contain any activation.

In~\autoref{fig:gestures_graphs_strobe}, we follow the same structure to show all the graphs of the Strobing attack in that same dataset. It can be observed that the strobing methodology reduces the number of poisoned frames needed for a successful attack, particularly when inserted at the end. Furthermore, this method does not significantly impact the clean accuracy of the models either.
We also follow that same structure for the two remaining datasets: cifar10-DVS, in~\autoref{fig:cifar_graphs} and~\autoref{fig:cifar_graphs_strobe}; and MNIST, in~\autoref{fig:mnist_graphs} and~\autoref{fig:mnist_graphs_strobe}.

A general tendency can be observed when comparing the results obtained with the DVS128-gesture dataset to those obtained for cifar10-DVS. While the performance on both ASR and clean accuracy remains consistent with previous results, it can be observed that a lower number of trigger frames is required to perform a successful attack in both \emph{Framed} (see~\autoref{fig:cifar_graphs}) and \emph{Strobing} (see~\autoref{fig:cifar_graphs_strobe}) methodologies, independently of the polarity or temporal position.

On the other hand, the NMNIST dataset presents more disparate results, as shown in~\autoref{fig:mnist_graphs} and~\autoref{fig:mnist_graphs_strobe}. The main difference compared to the other two datasets is that smaller triggers cannot perform the attack with polarity $p=0$; the hypothesis is that the lower amounts of noise in the samples make it even more difficult for the model to discern the trigger in the frames. However, when the trigger is inserted at the start or middle of the sample with any other polarities, very high ASR values are observed with minimal decrease in clean accuracy. Comparing both attack methodologies, similar tendencies to other datasets can be observed. Generally, there is no downside to including the clean frame between the triggers, but it results in a significant improvement when the trigger is inserted at the end of the sample.

After seeing these results, we selected the DVS128-gesture as our primary dataset to test the procedures and defenses typical of DL and attacks in physical scenarios. Indeed, this dataset represents the worst-case scenario, being the most challenging one to attack among the tested.

% \begin{figure*}[!ht]
%     \centering

%     \begin{subfigure}[b]{0.49\linewidth}
%         \includegraphics[width=\linewidth]{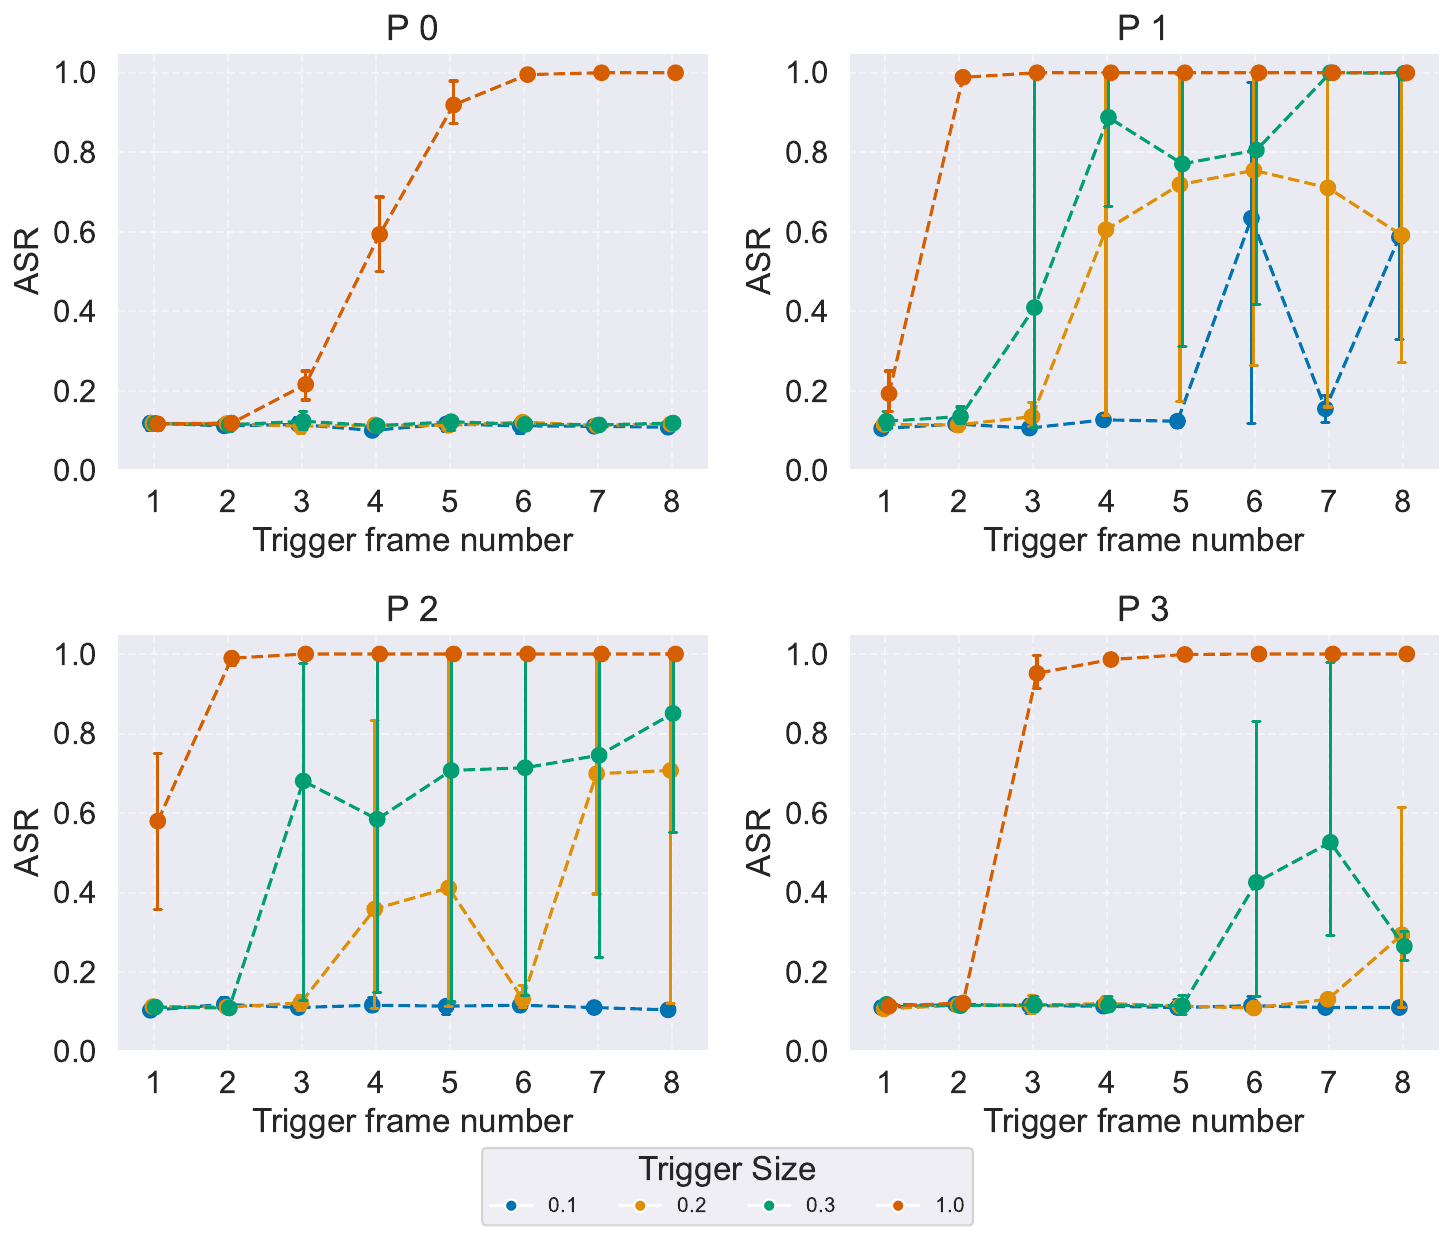}
%         \caption{ASR Start position}
%     \end{subfigure}
%     \hfill
%     \begin{subfigure}[b]{0.49\linewidth}
%         \includegraphics[width=\linewidth]{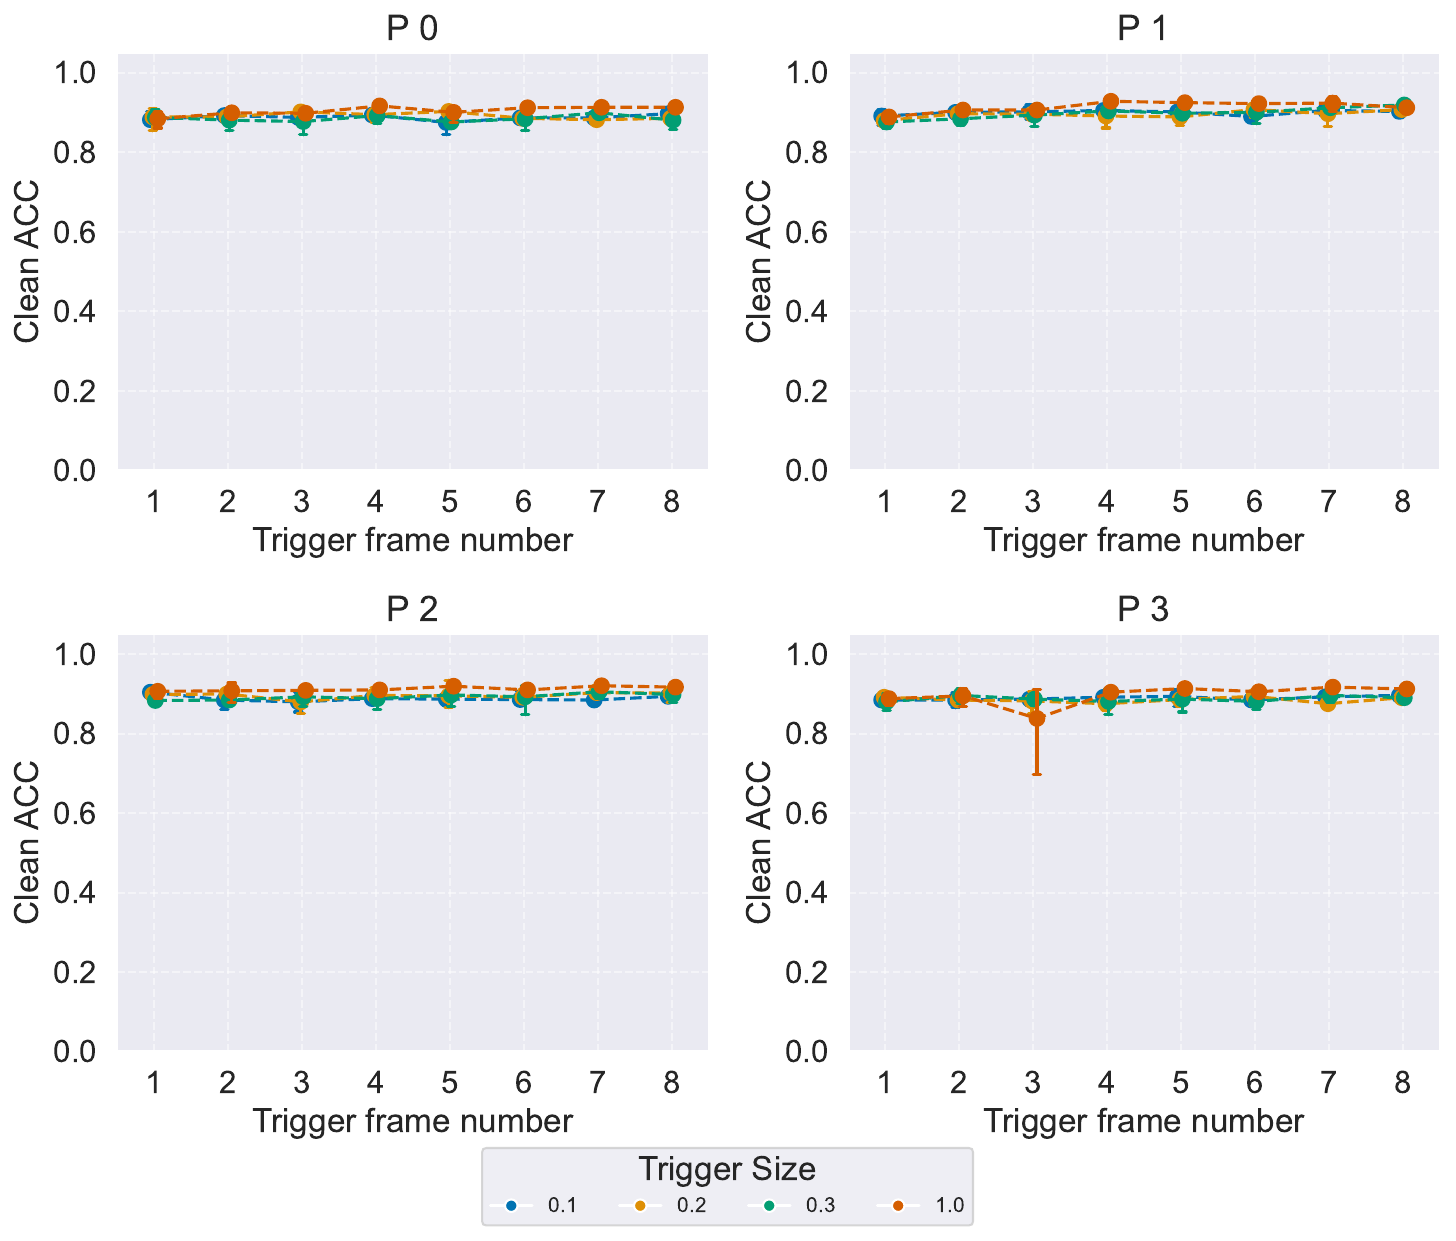}
%         \caption{Clean ACC Start Position}
%     \end{subfigure}
    
%     \begin{subfigure}[b]{0.49\linewidth}
%         \includegraphics[width=\linewidth]{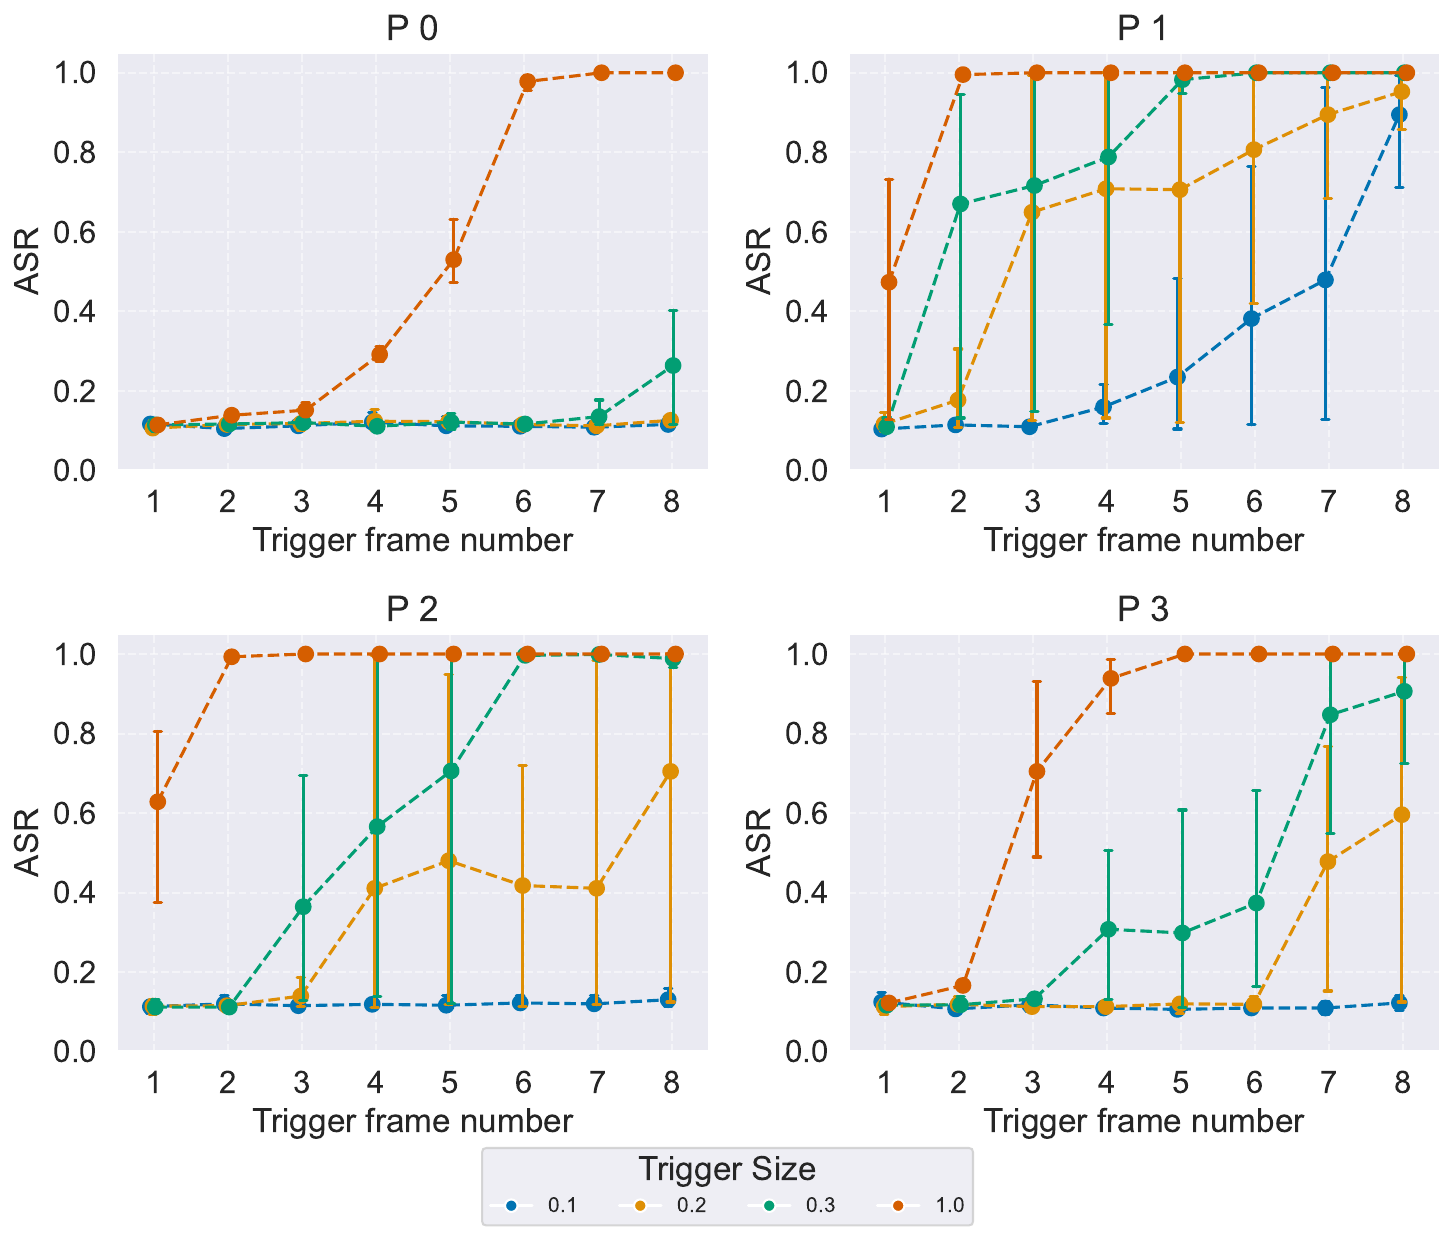}
%         \caption{ASR Mid position}
%     \end{subfigure}
%     % \hfill
%     % \begin{subfigure}[b]{0.49\linewidth}
%     %     \includegraphics[width=\linewidth]{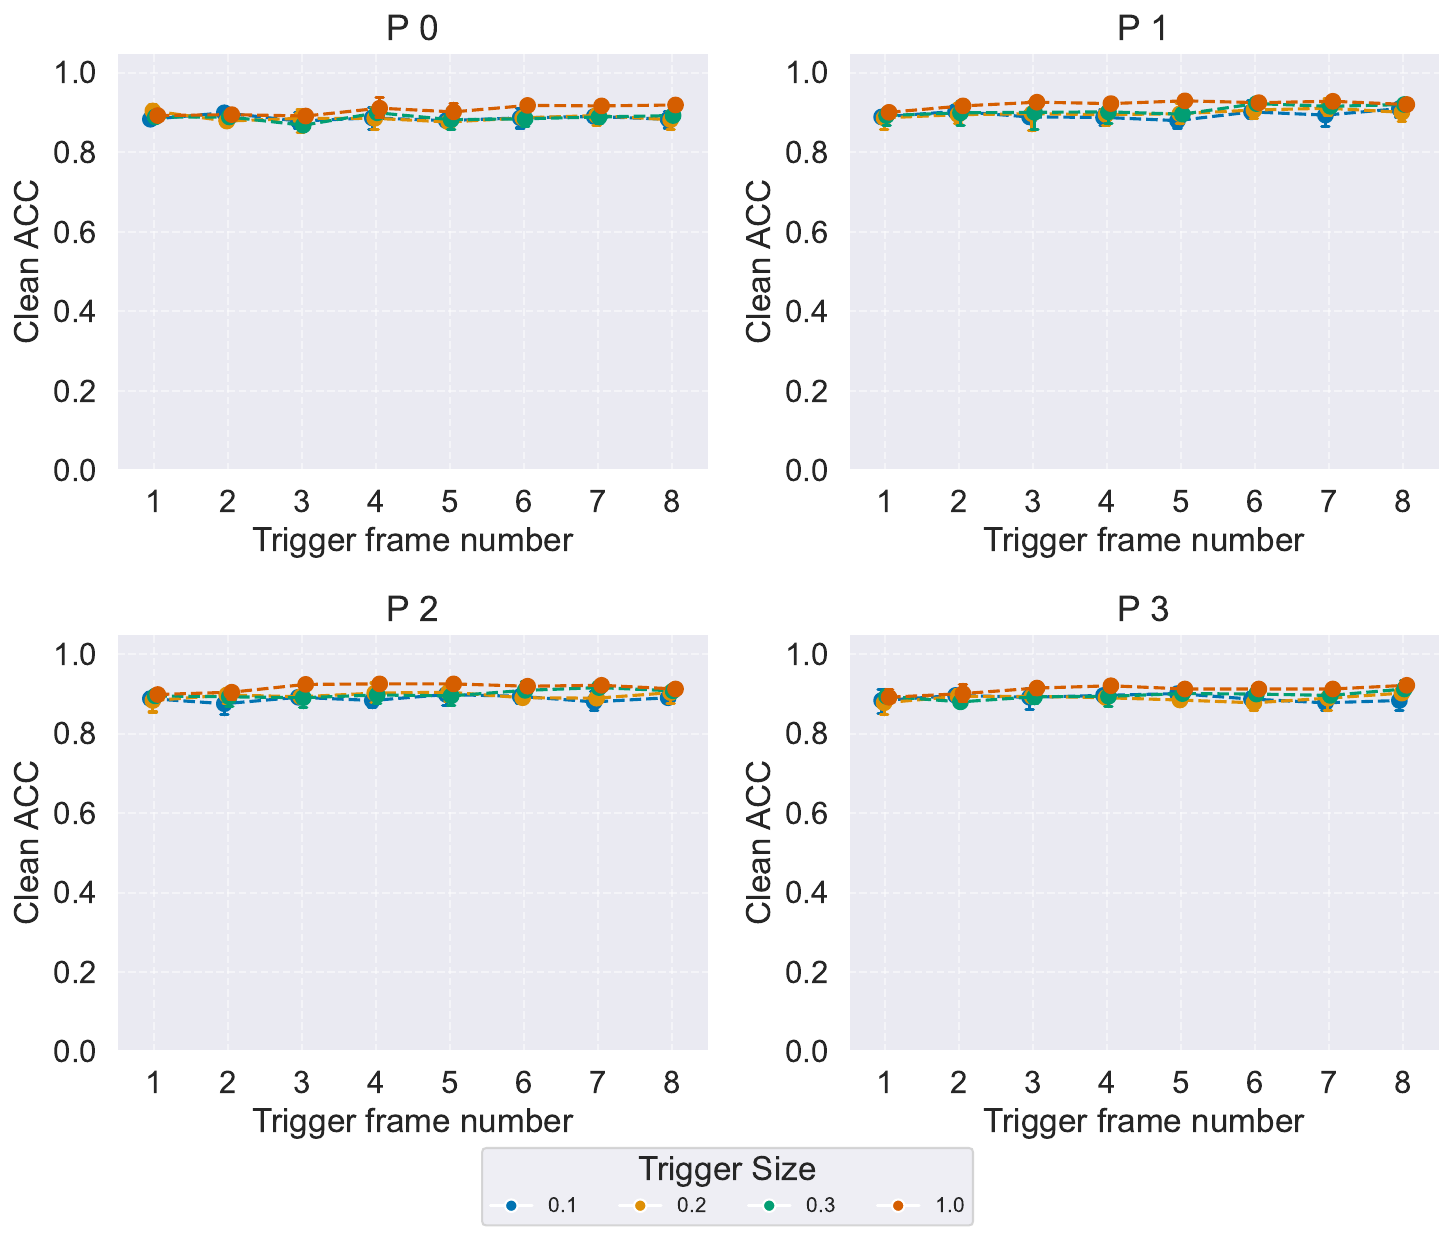}
%     %     \caption{Clean ACC Mid Position}
%     % \end{subfigure}

%     \begin{subfigure}[b]{0.49\linewidth}
%         \includegraphics[width=\linewidth]{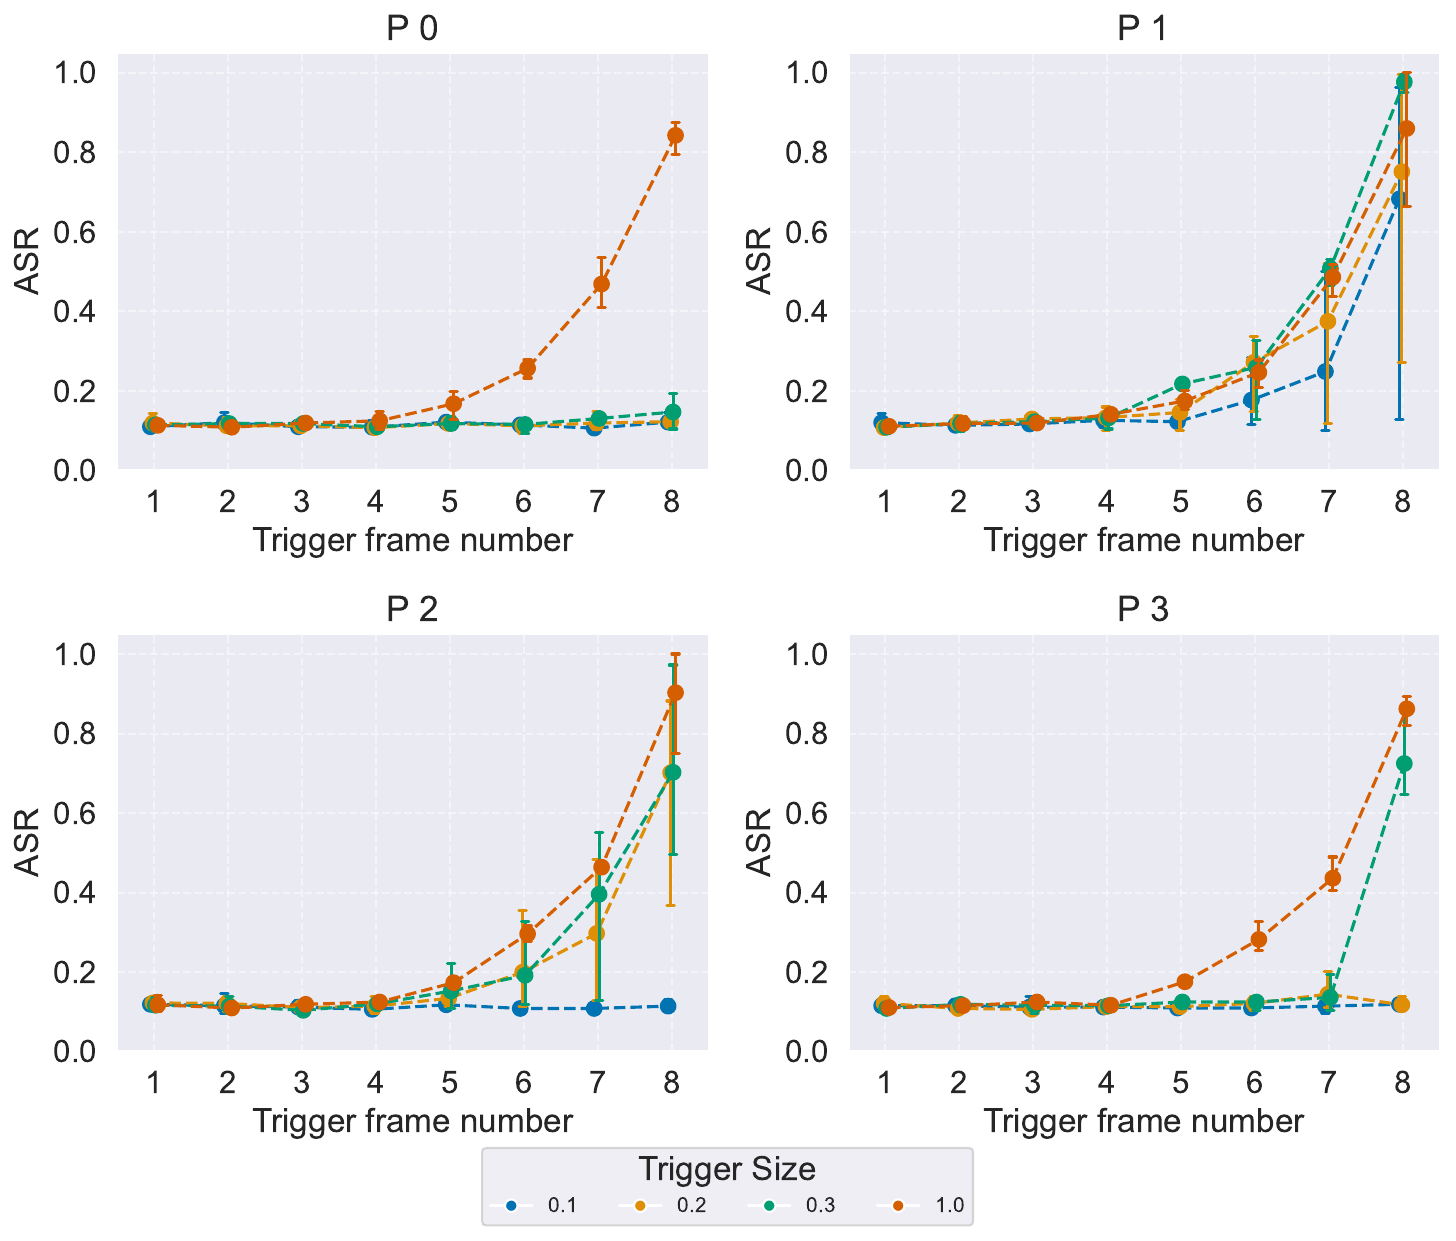}
%         \caption{ASR End position}
%     \end{subfigure}
%     % \hfill
%     % \begin{subfigure}[b]{0.49\linewidth}
%     %     \includegraphics[width=\linewidth]{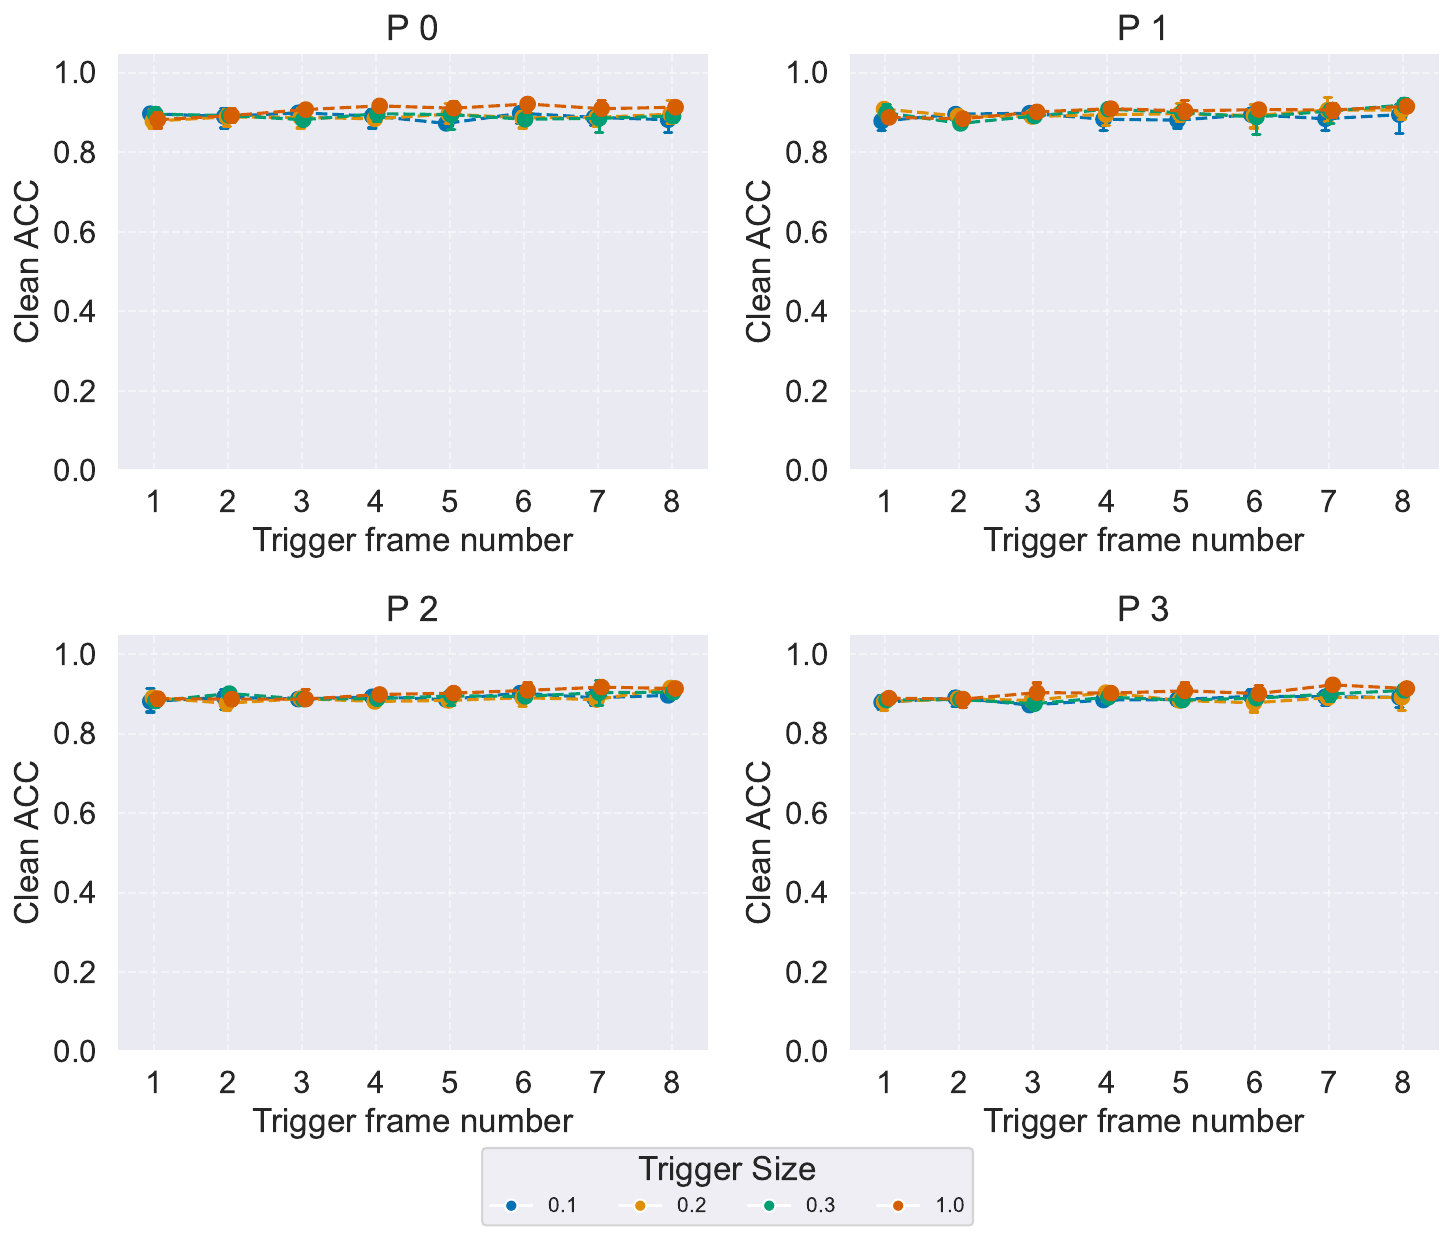}
%     %     \caption{Clean ACC End Position}
%     % \end{subfigure}
    
%     \caption{All graphs containing ASR and Clean accuracy for the DVS128-gesture dataset with continuous triggers.}
%     \label{fig:gestures_graphs}
% \end{figure*}

\begin{figure*}[!ht]
    \centering

    \begin{subfigure}[b]{0.49\linewidth}
        \includegraphics[width=\linewidth]{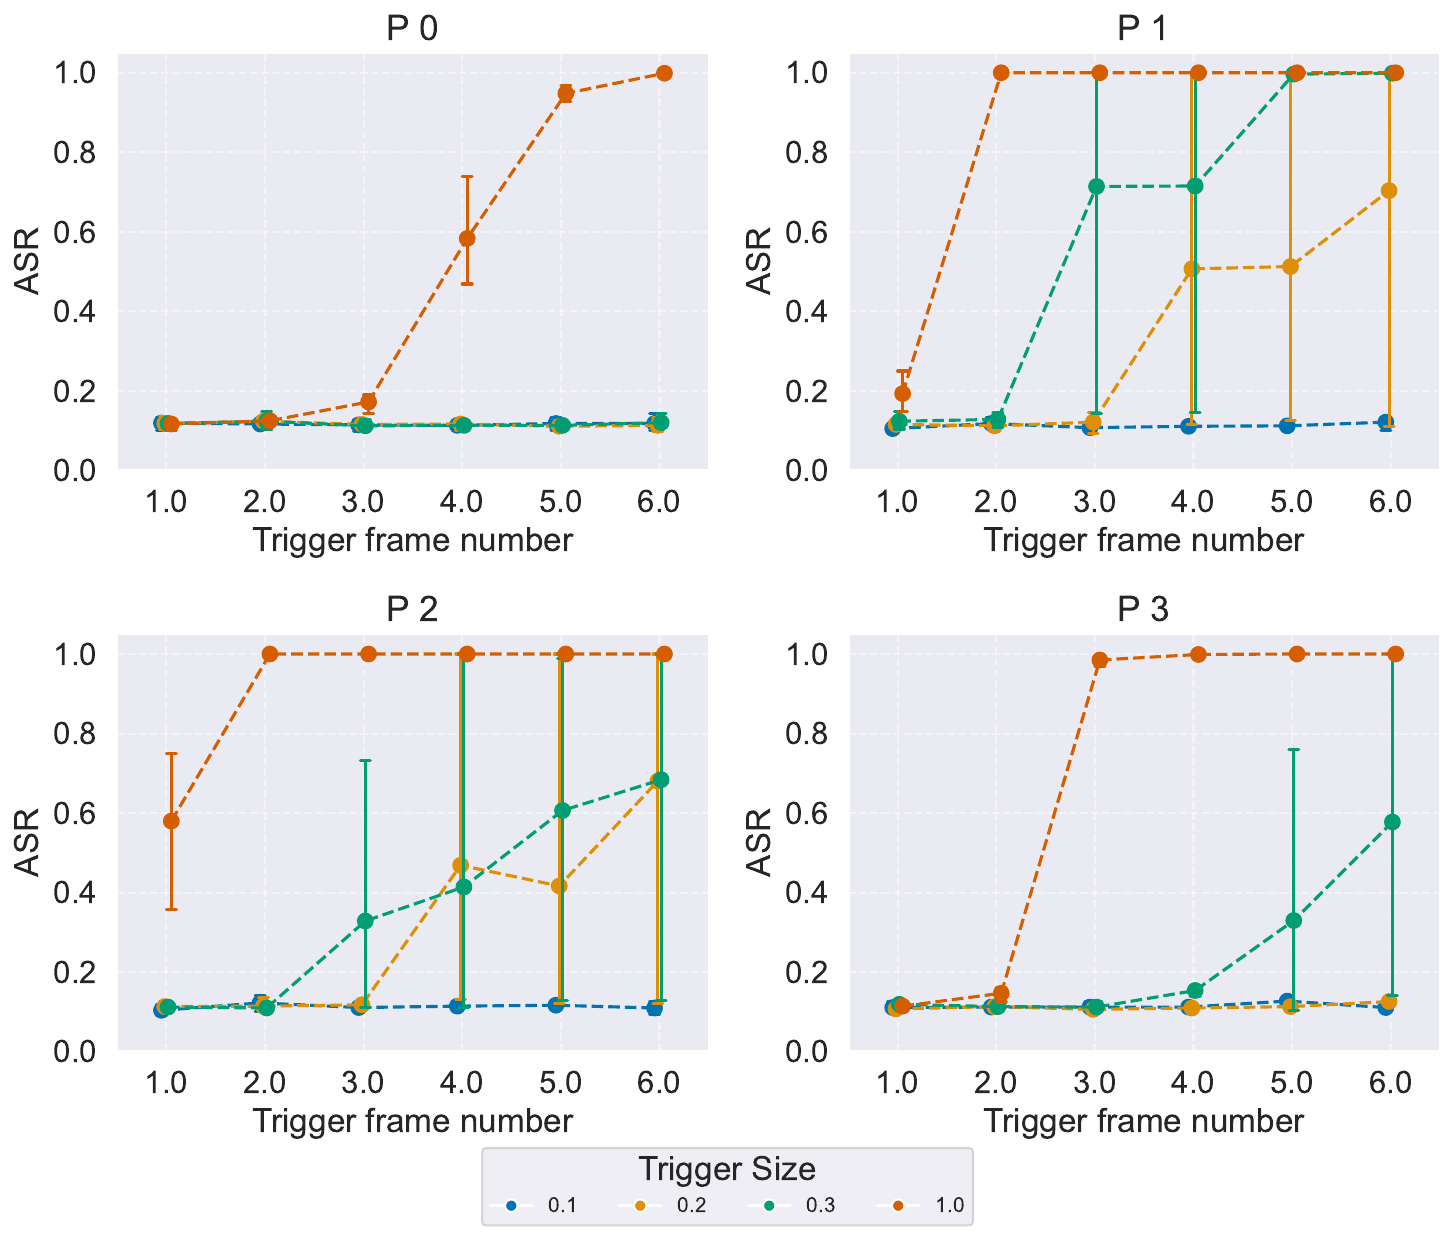}
        \caption{ASR Start position}
    \end{subfigure}
    \hfill
    \begin{subfigure}[b]{0.49\linewidth}
        \includegraphics[width=\linewidth]{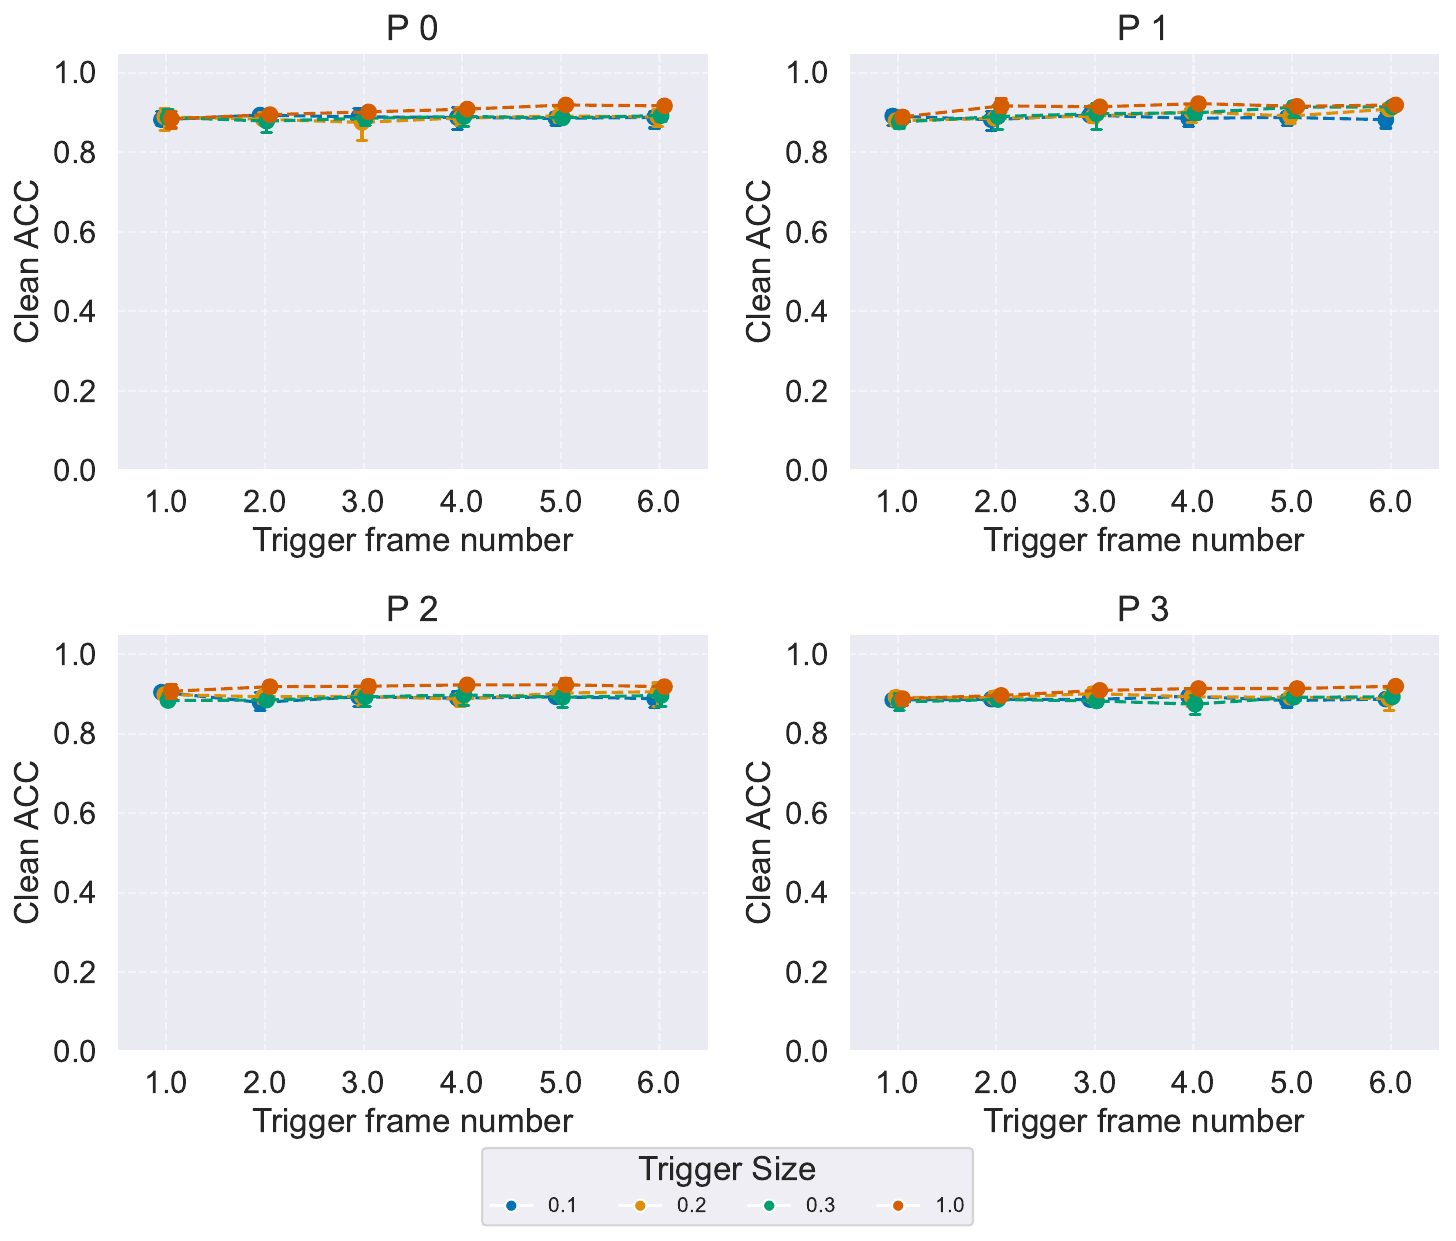}
        \caption{Clean ACC Start Position}
    \end{subfigure}
    
    \begin{subfigure}[b]{0.49\linewidth}
        \includegraphics[width=\linewidth]{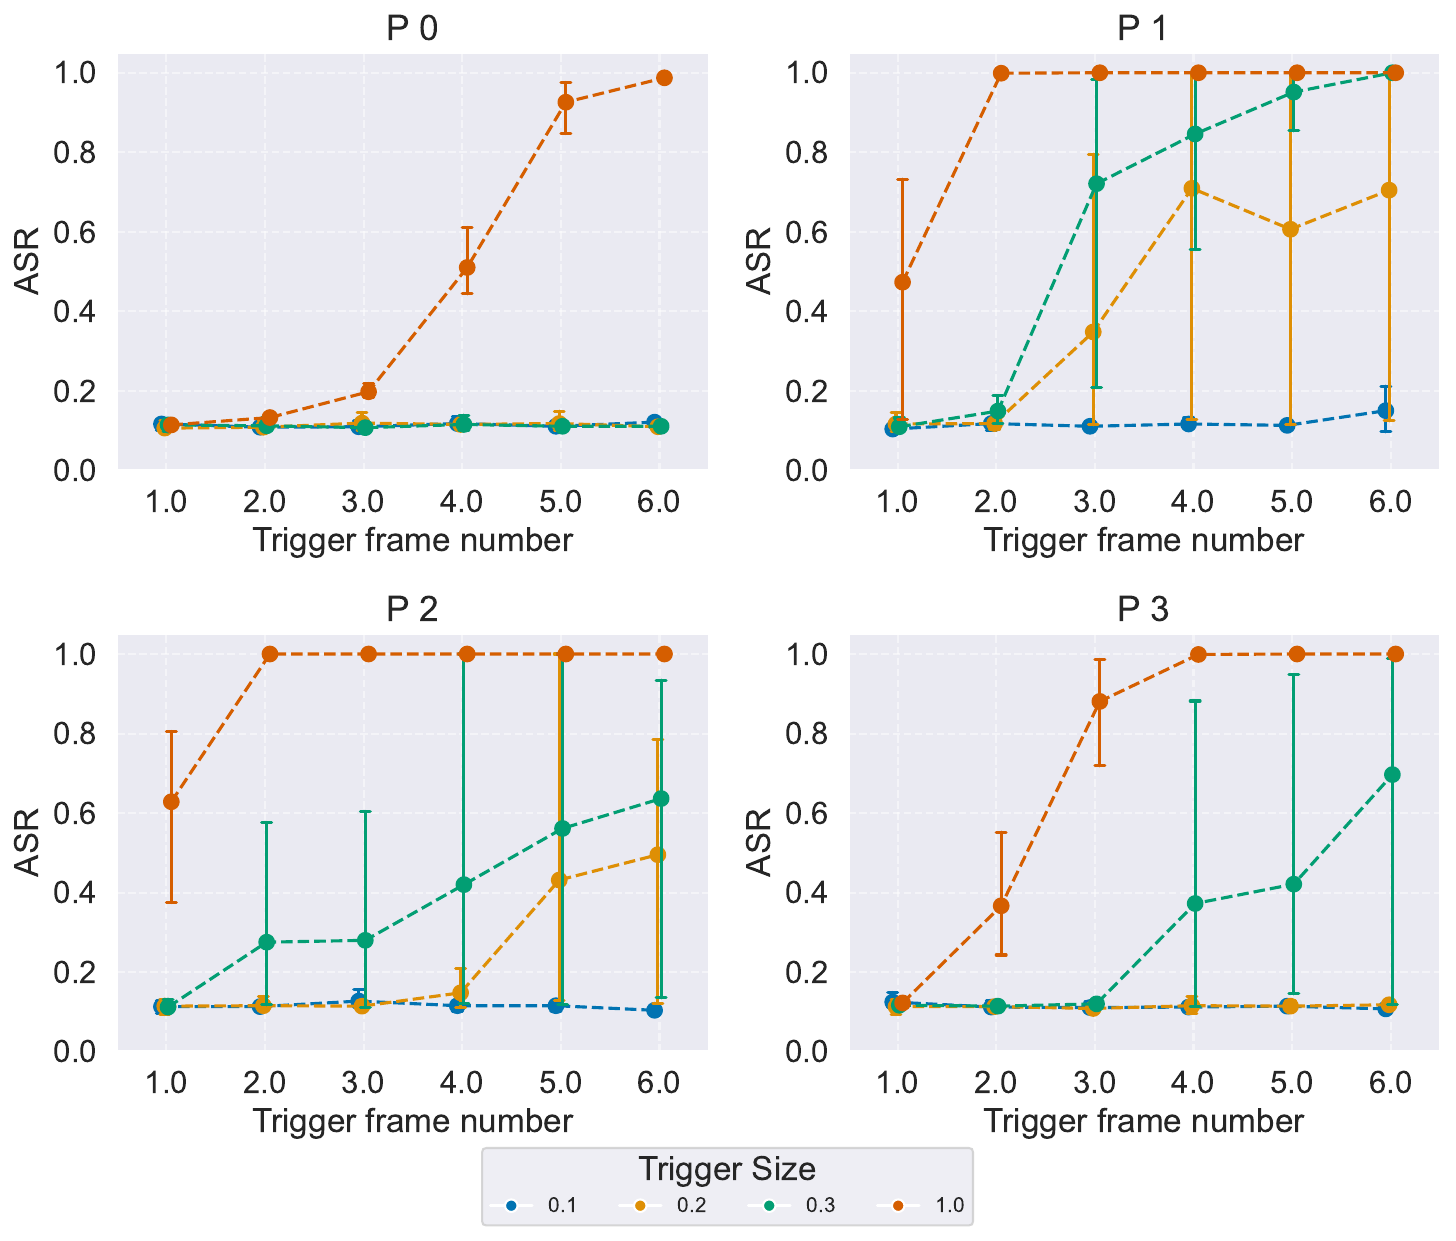}
        \caption{ASR Mid position}
    \end{subfigure}
    \hfill
    % \begin{subfigure}[b]{0.49\linewidth}
    %     \includegraphics[width=\linewidth]{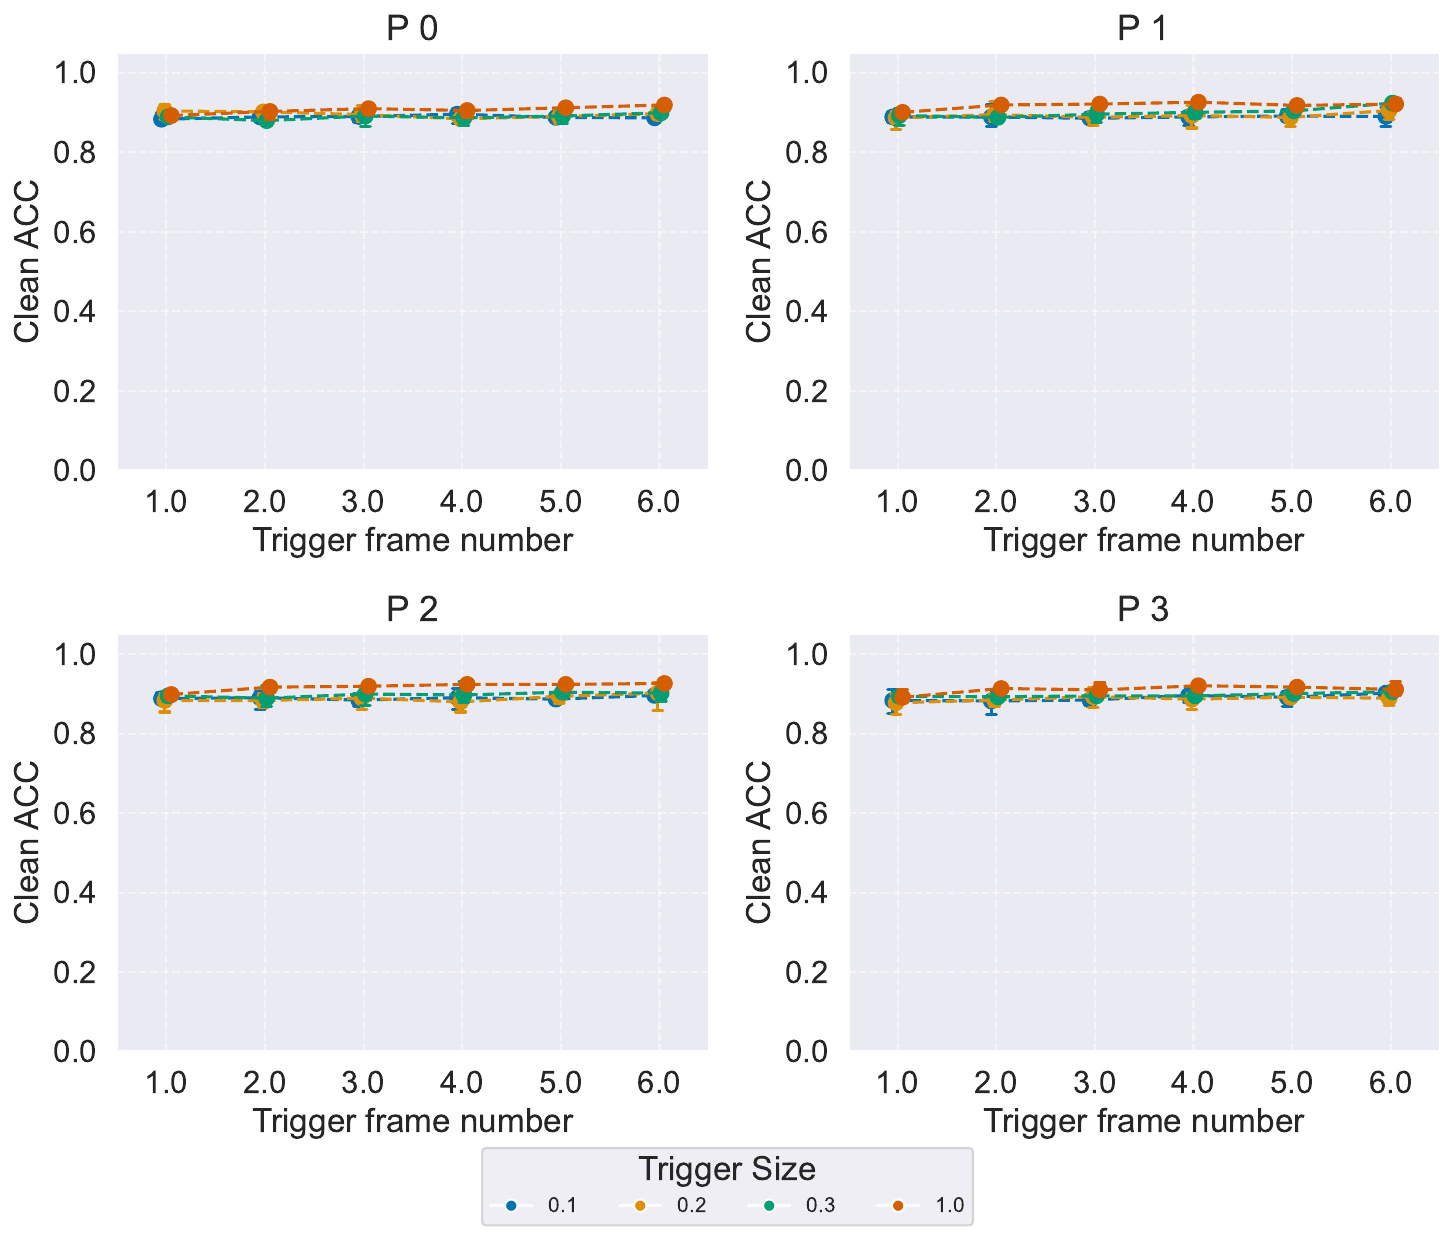}
    %     \caption{Clean ACC Mid Position}
    % \end{subfigure}
    \begin{subfigure}[b]{0.49\linewidth}
        \includegraphics[width=\linewidth]{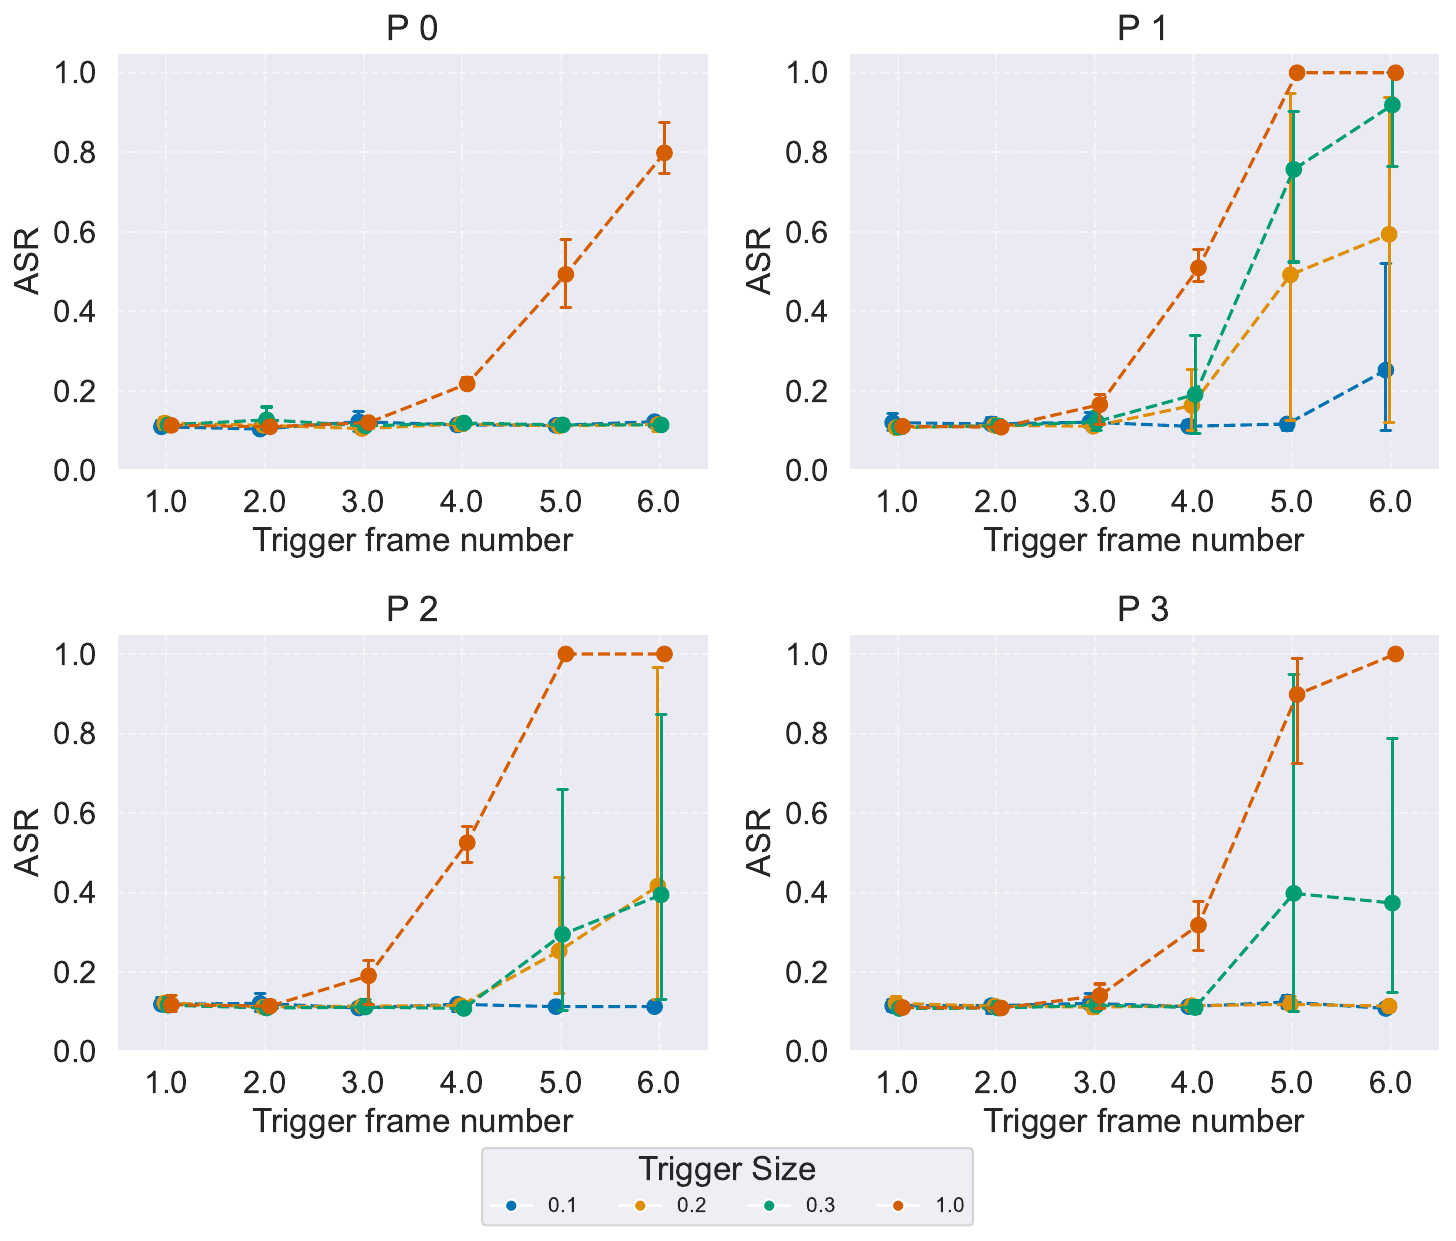}
        \caption{ASR End position}
    \end{subfigure}
    % \hfill
    % \begin{subfigure}[b]{0.49\linewidth}
    %     \includegraphics[width=\linewidth]{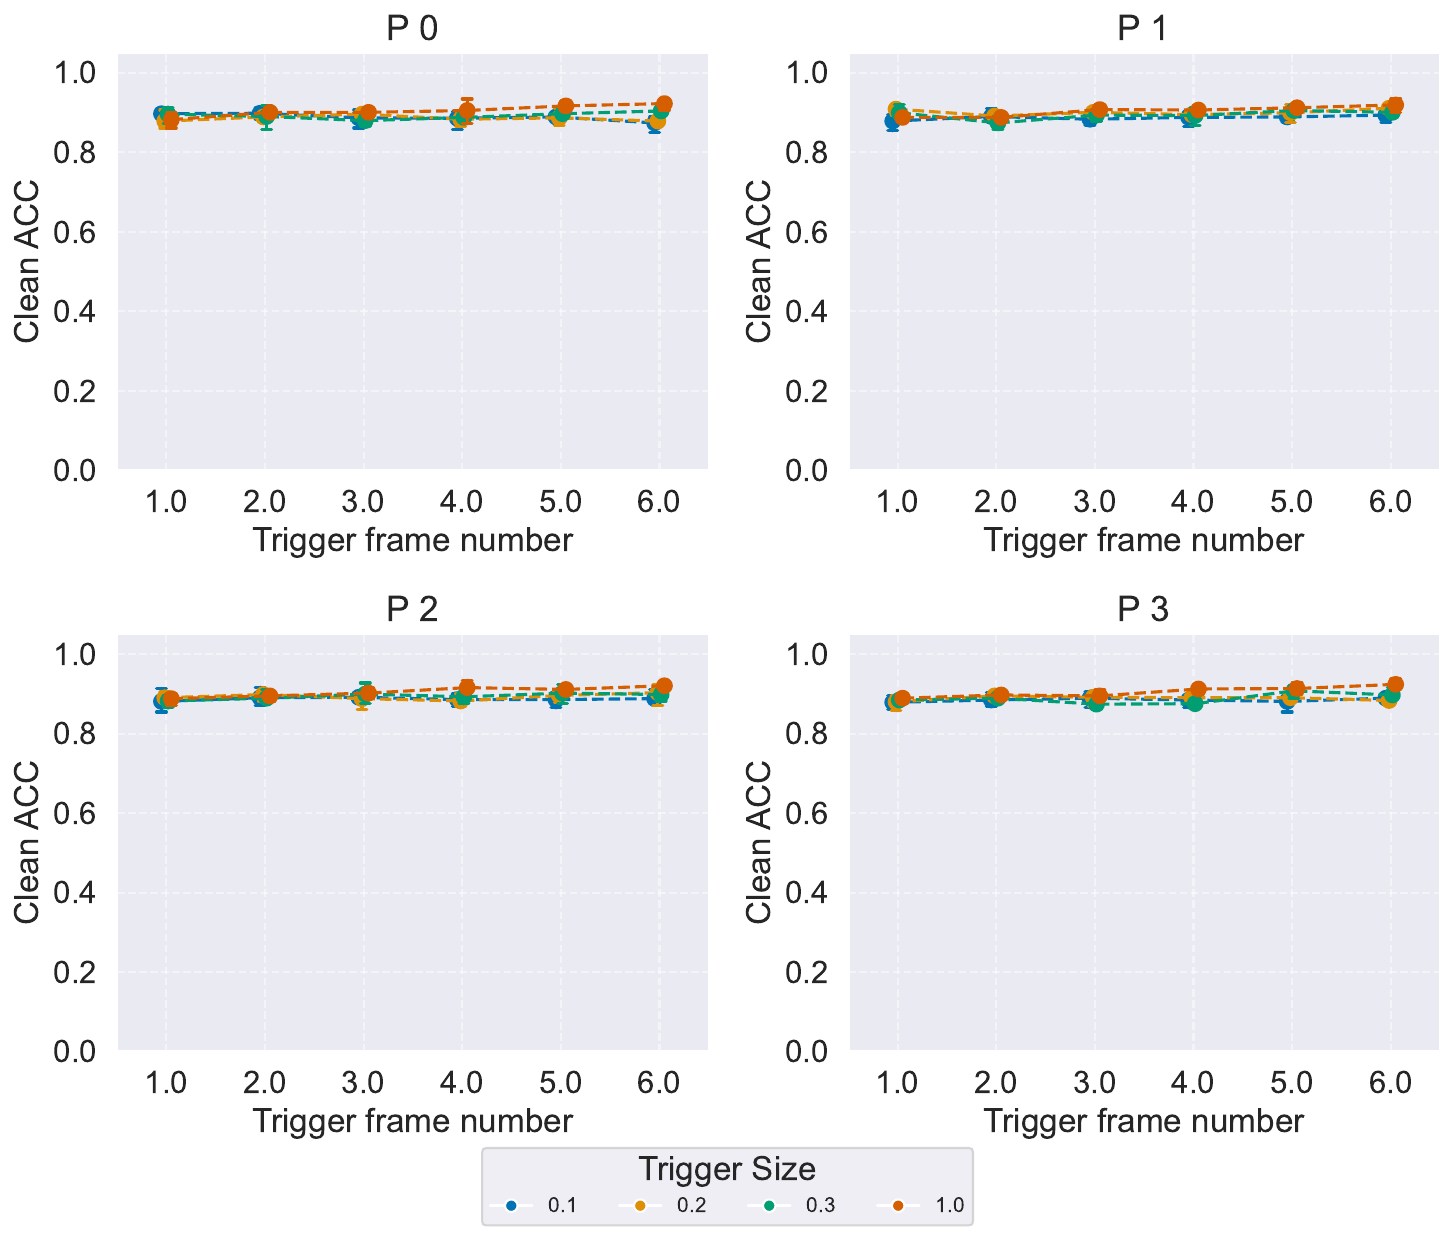}
    %     \caption{Clean ACC End Position}
    % \end{subfigure}
    
    \caption{All graphs containing ASR and Clean accuracy for the DVS128-gesture dataset with strobing triggers with a single frame of clean gap.}
    \label{fig:gestures_graphs_strobe}
\end{figure*}

% \begin{figure*}[!ht]
%     \centering

%     \begin{subfigure}[b]{0.49\linewidth}
%         \includegraphics[width=\linewidth]{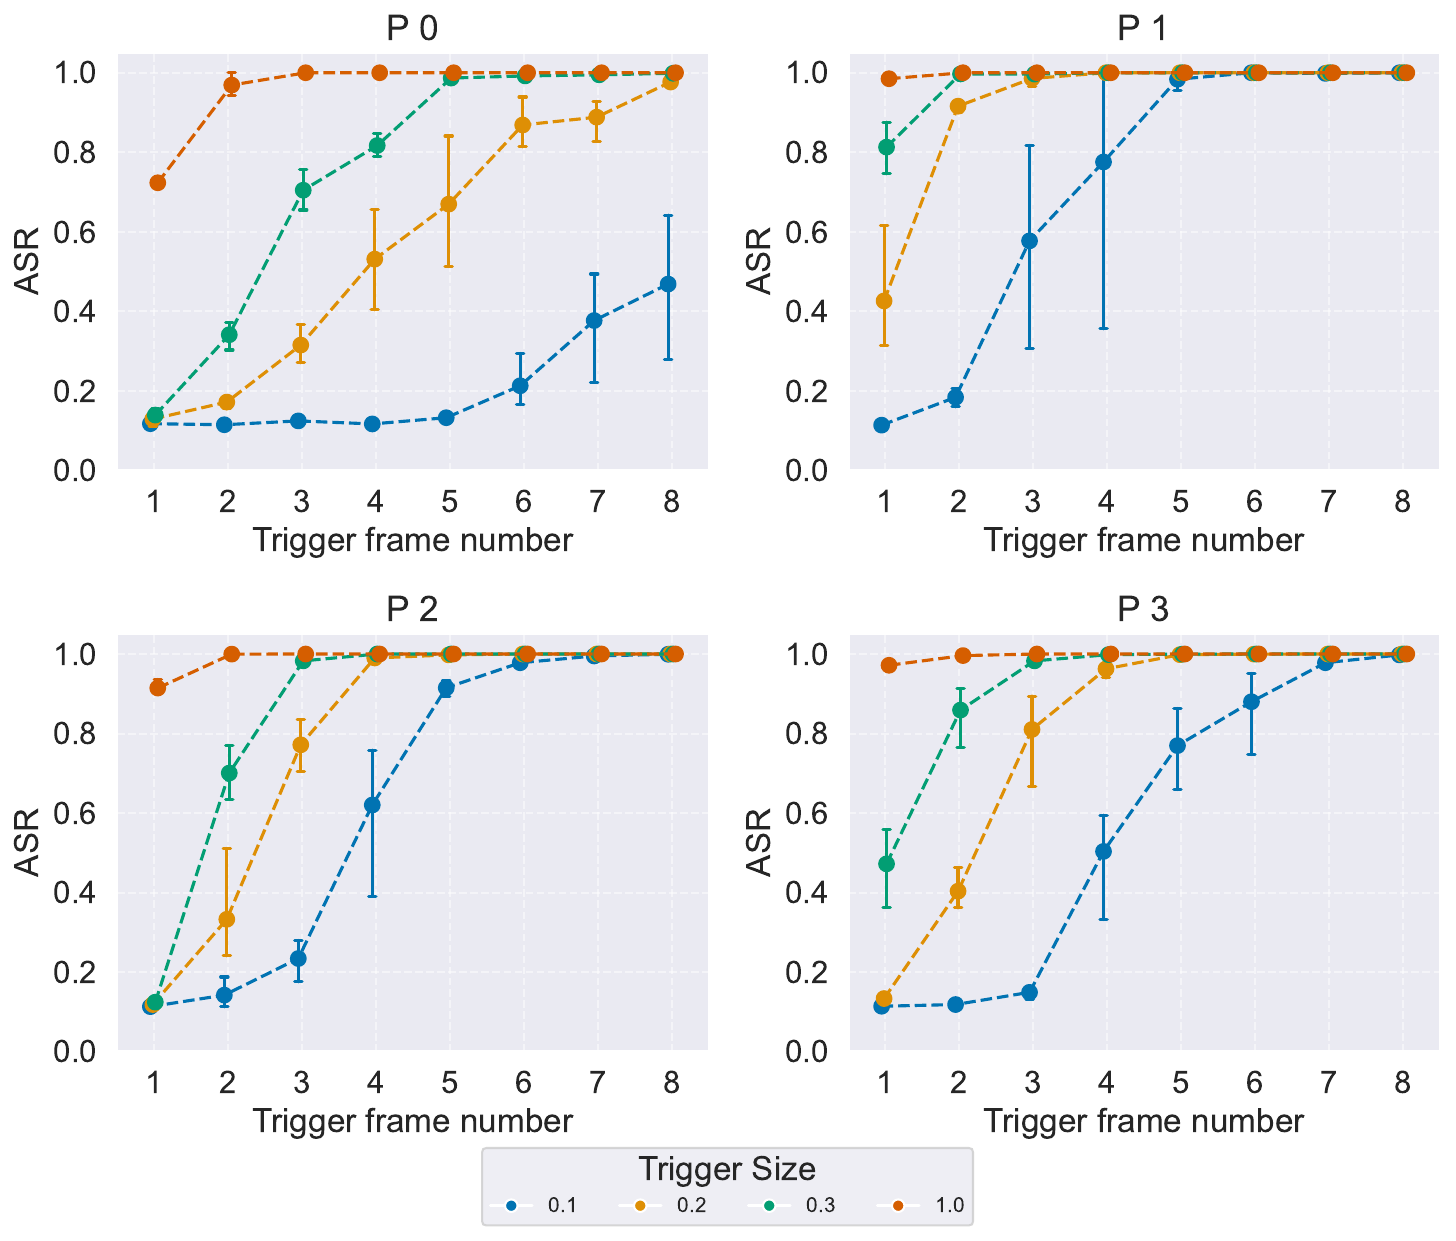}
%         \caption{ASR Start position}
%     \end{subfigure}
%     \hfill
%     \begin{subfigure}[b]{0.49\linewidth}
%         \includegraphics[width=\linewidth]{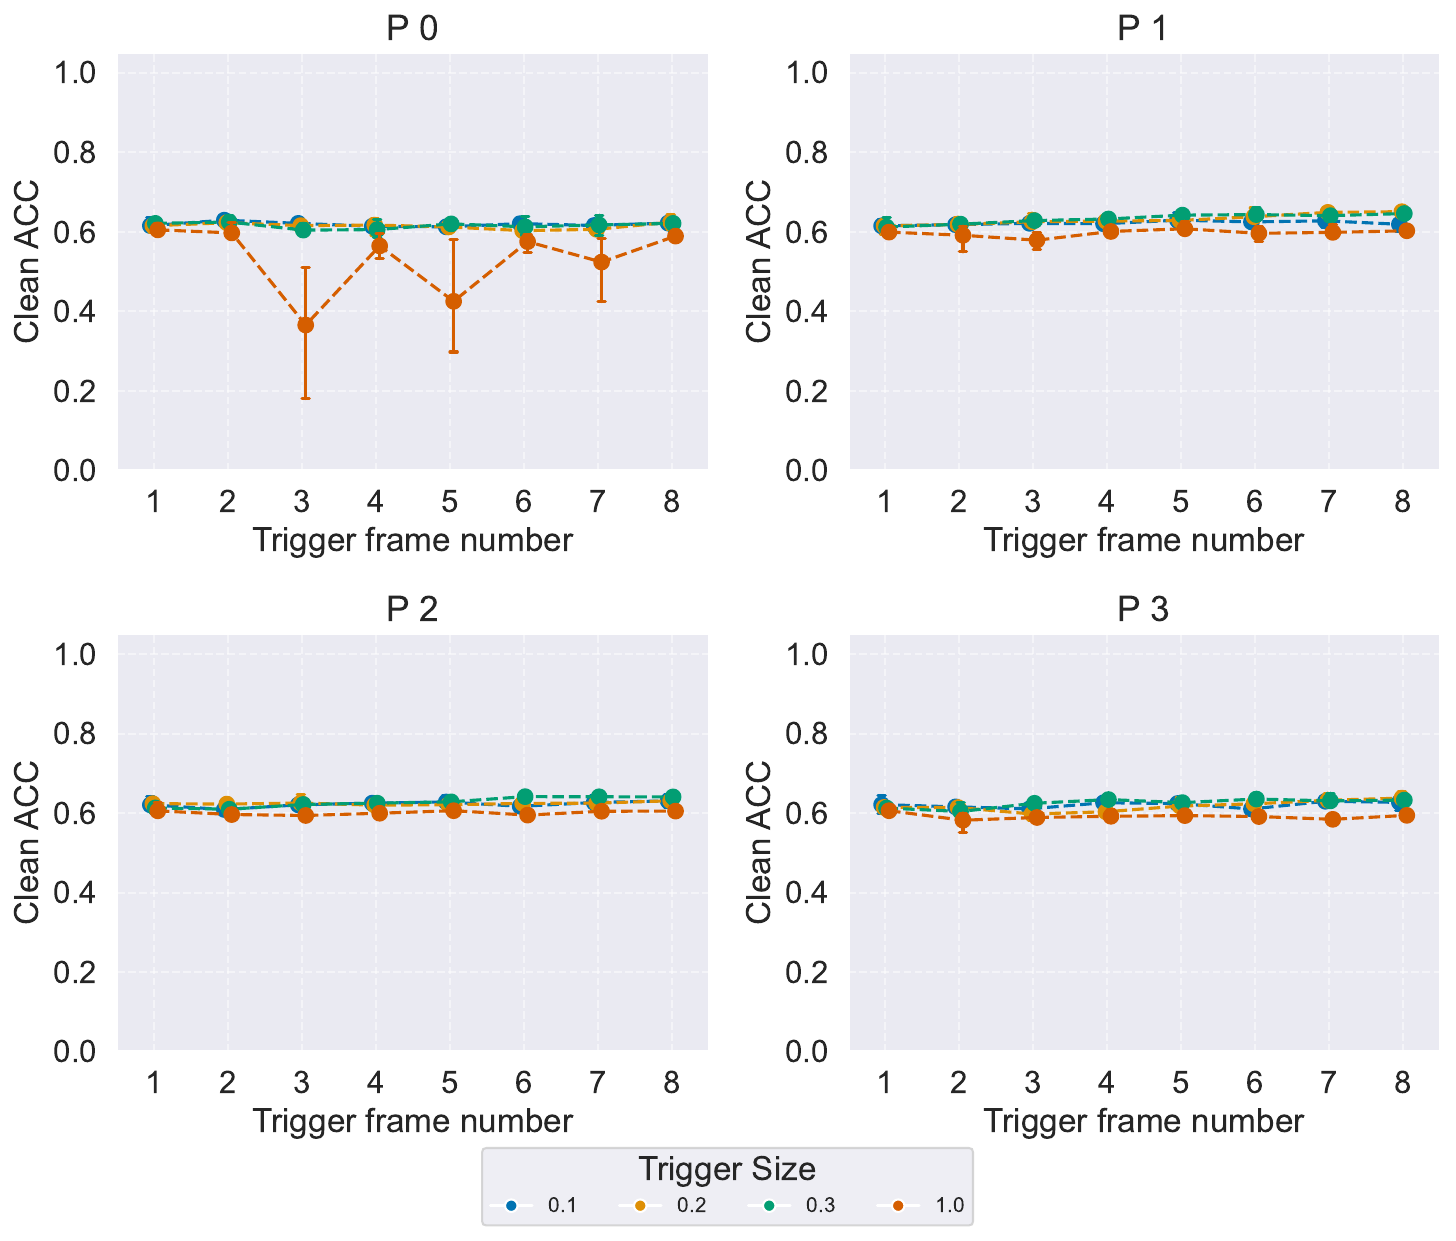}
%         \caption{Clean ACC Start Position}
%     \end{subfigure}
    
%     \begin{subfigure}[b]{0.49\linewidth}
%         \includegraphics[width=\linewidth]{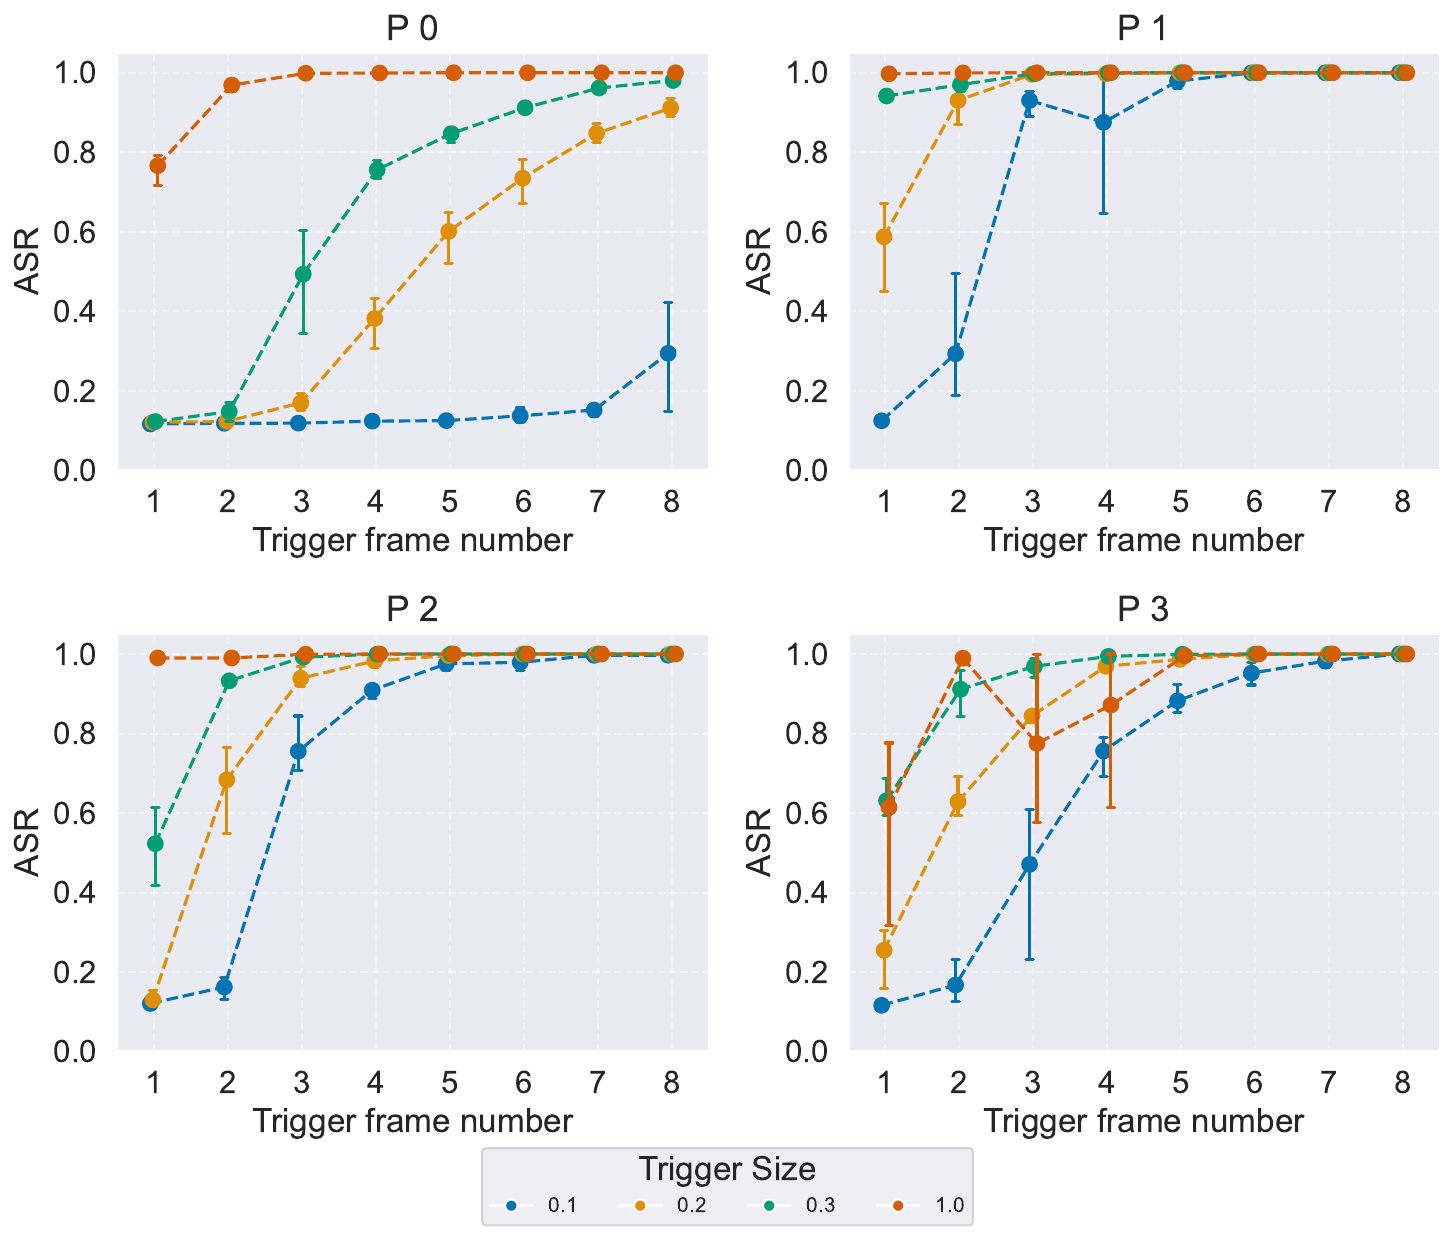}
%         \caption{ASR Mid position}
%     \end{subfigure}
%     \hfill
%     \begin{subfigure}[b]{0.49\linewidth}
%         \includegraphics[width=\linewidth]{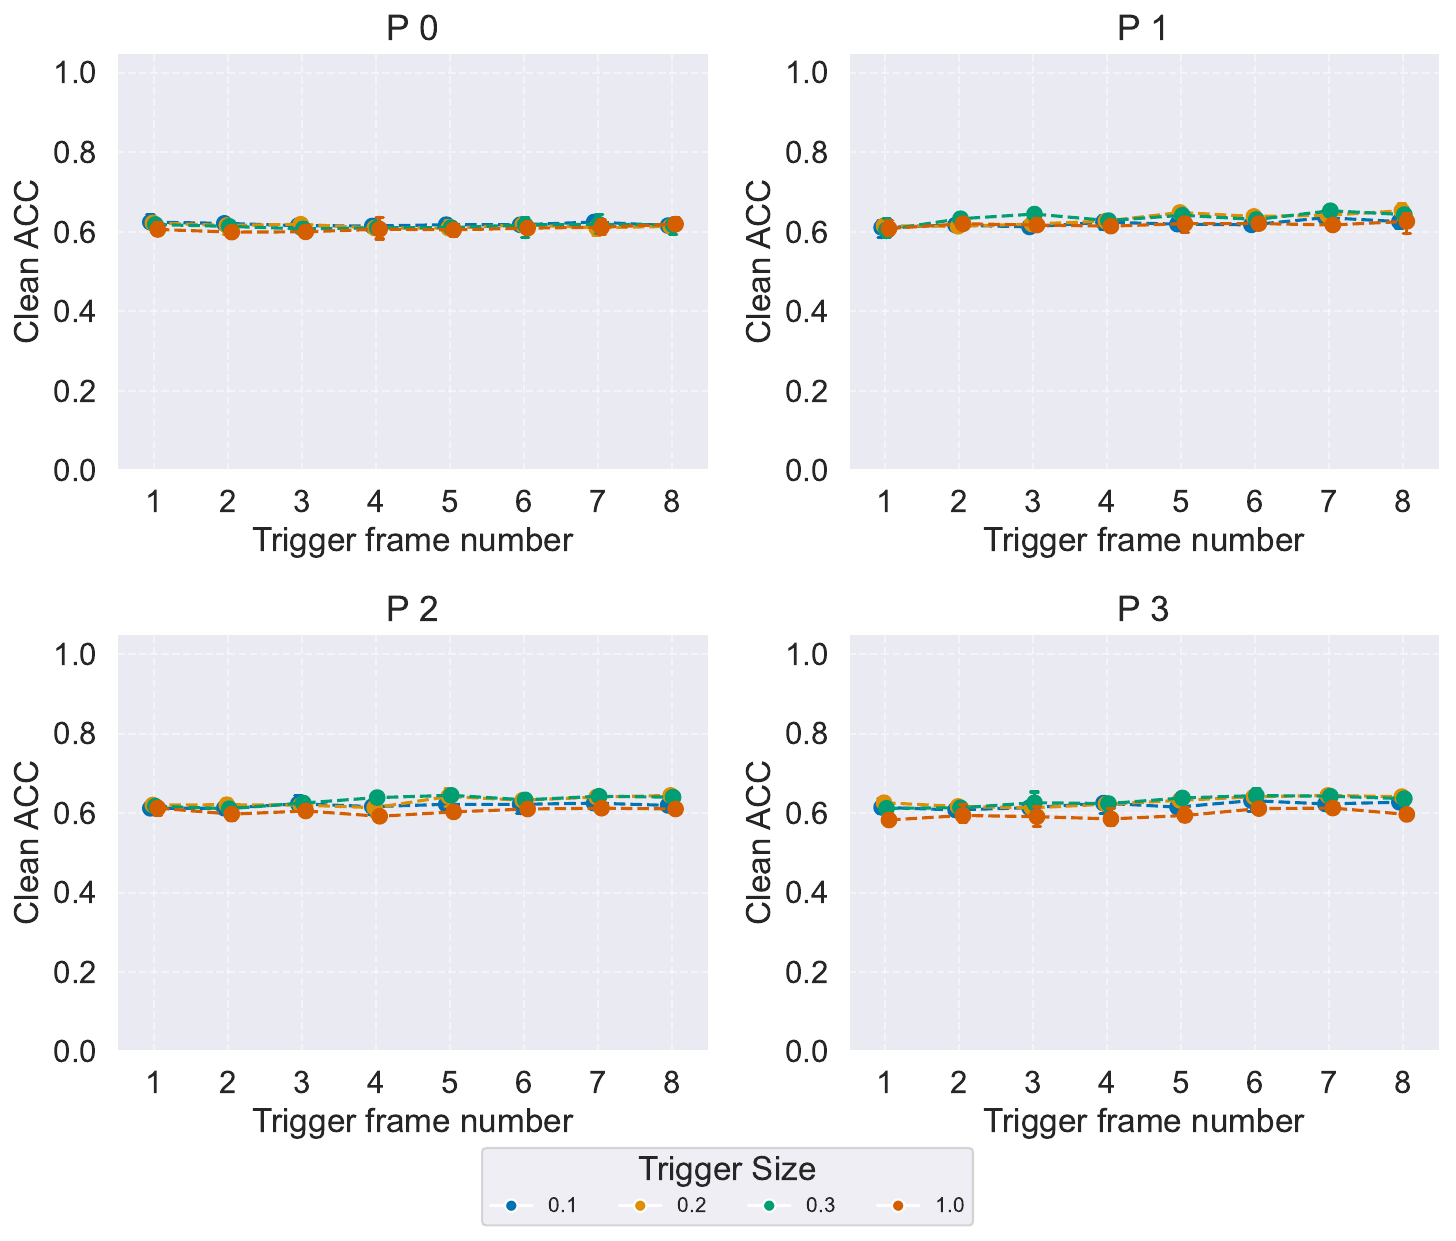}
%         \caption{Clean ACC Mid Position}
%     \end{subfigure}

%     \begin{subfigure}[b]{0.49\linewidth}
%         \includegraphics[width=\linewidth]{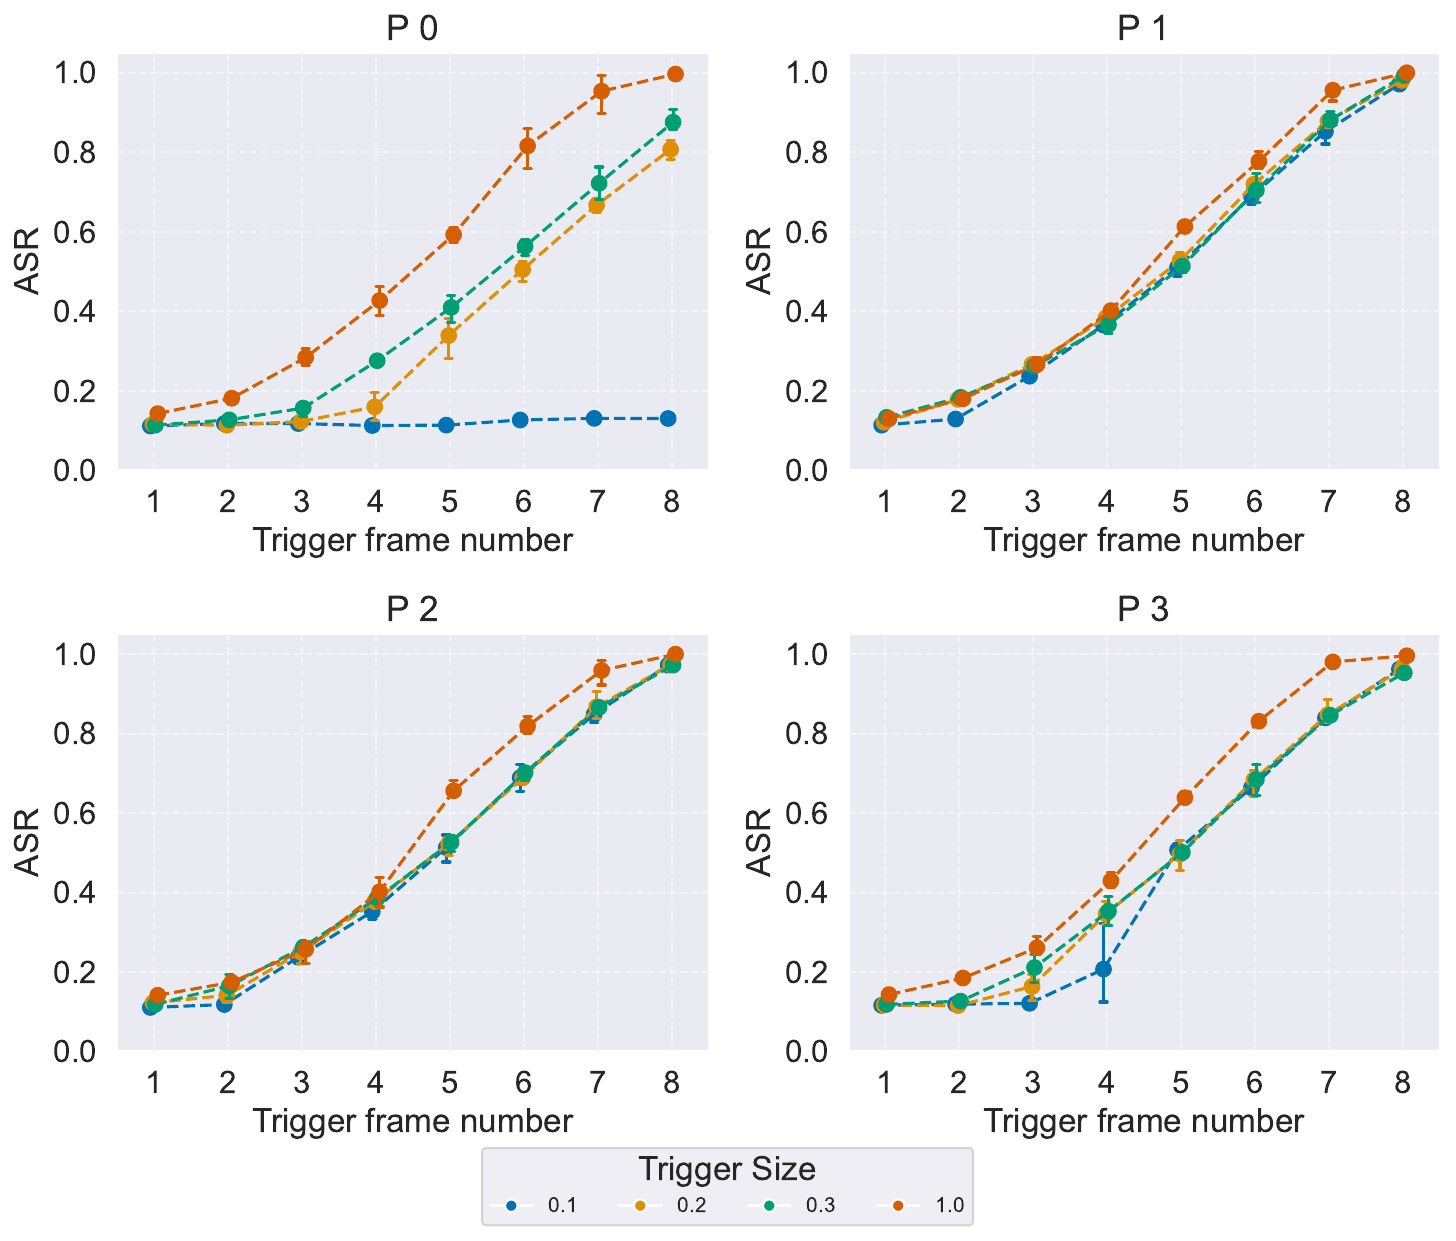}
%         \caption{ASR End position}
%     \end{subfigure}
%     \hfill
%     \begin{subfigure}[b]{0.49\linewidth}
%         \includegraphics[width=\linewidth]{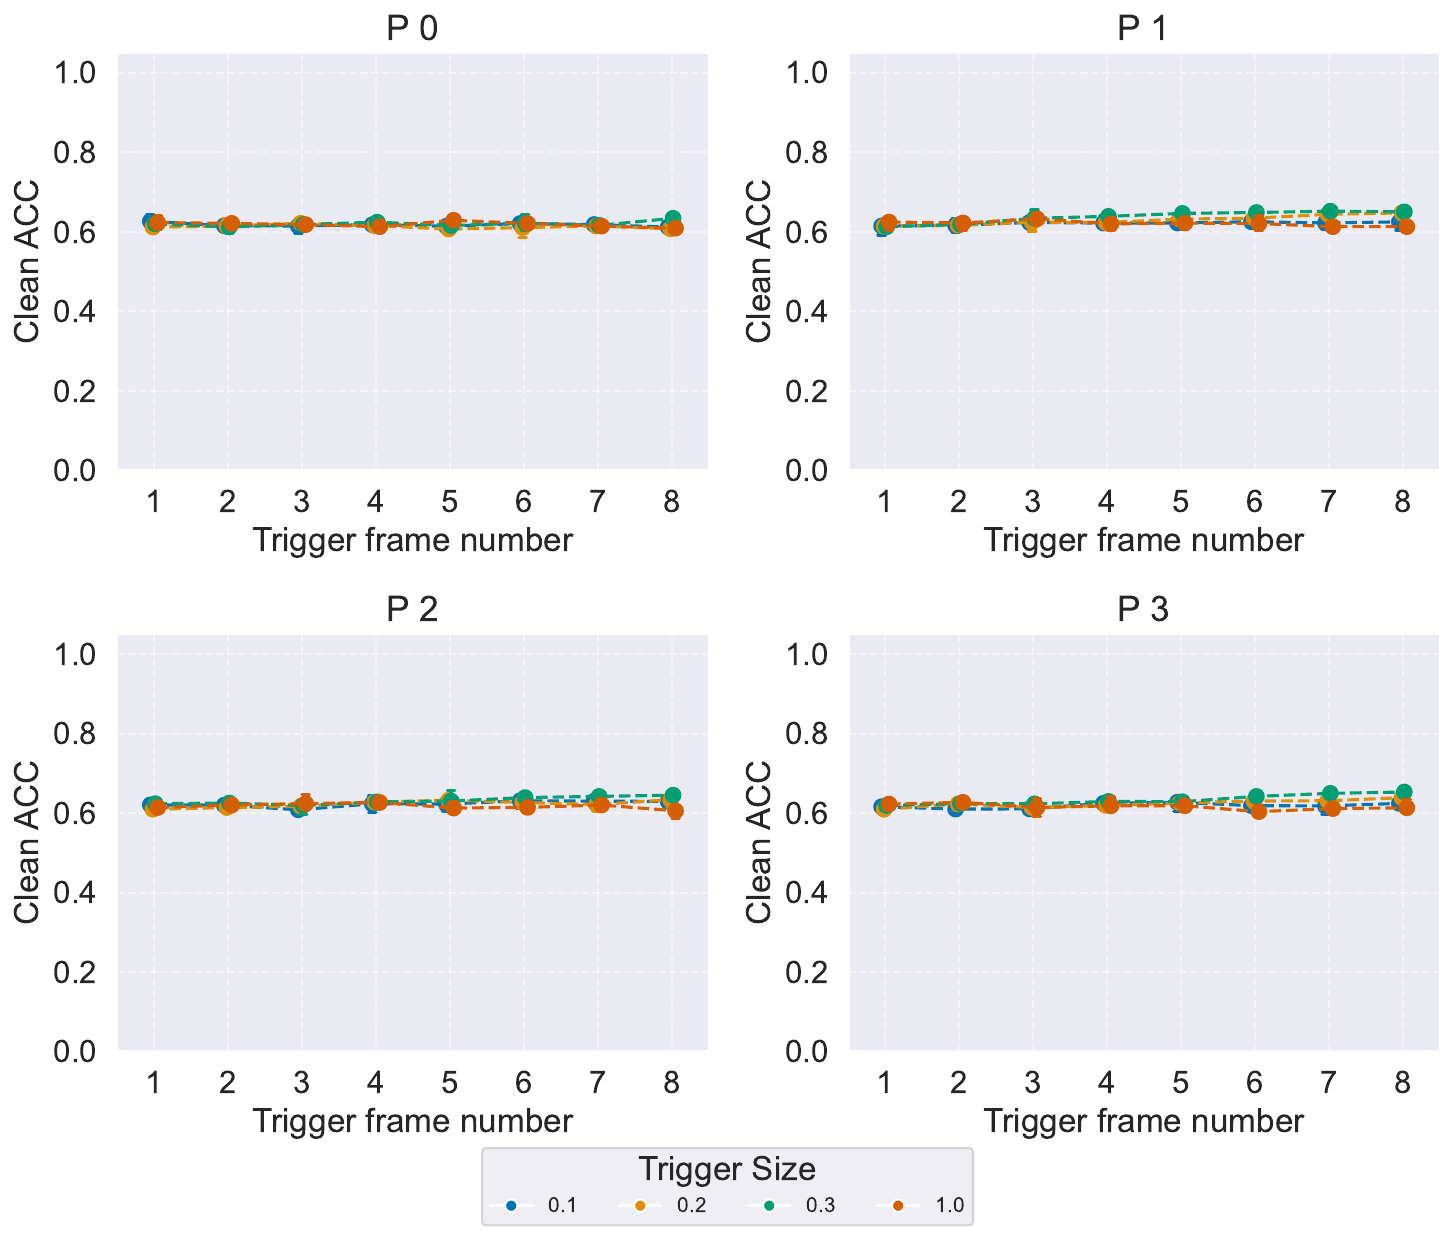}
%         \caption{Clean ACC End Position}
%     \end{subfigure}
    
%     \caption{All graphs containing ASR and Clean accuracy for the cifar10-DVS dataset with continuous triggers.}
%     \label{fig:cifar_graphs}
% \end{figure*}

\begin{figure*}[!ht]
    \centering

    \begin{subfigure}[b]{0.49\linewidth}
        \includegraphics[width=\linewidth]{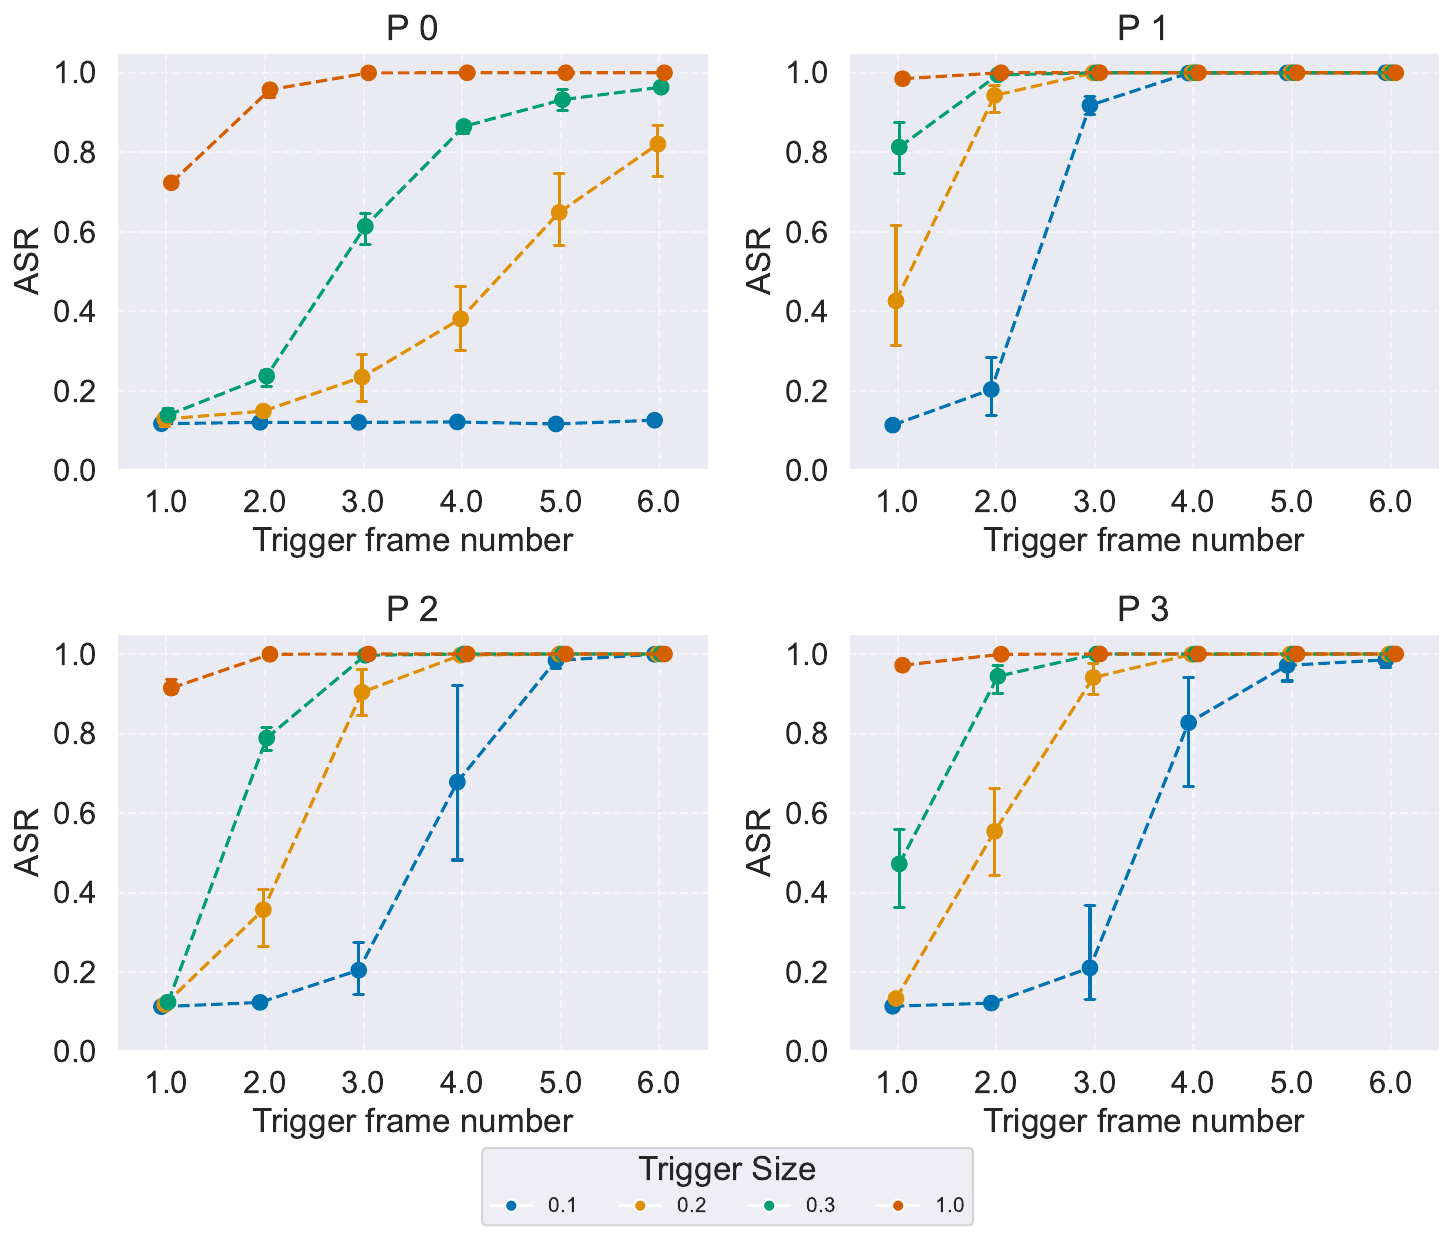}
        \caption{ASR Start position}
    \end{subfigure}
    \hfill
    \begin{subfigure}[b]{0.49\linewidth}
        \includegraphics[width=\linewidth]{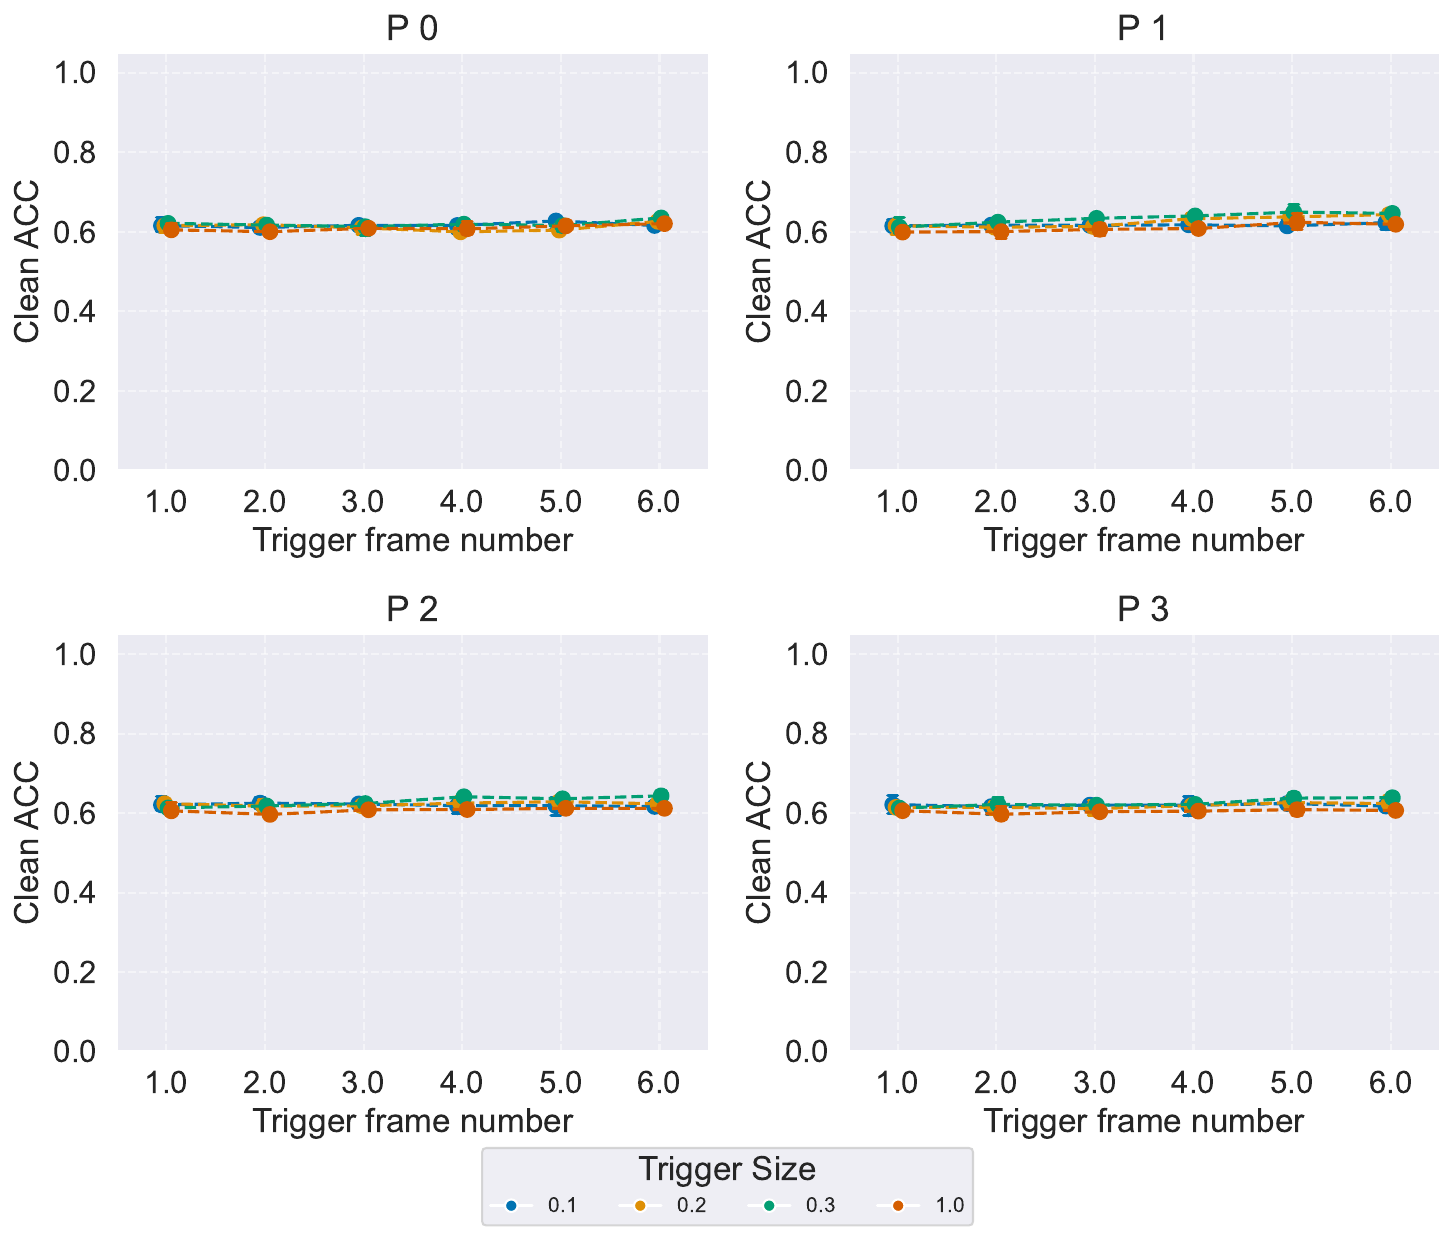}
        \caption{Clean ACC Start Position}
    \end{subfigure}
    
    % \begin{subfigure}[b]{0.49\linewidth}
    %     \includegraphics[width=\linewidth]{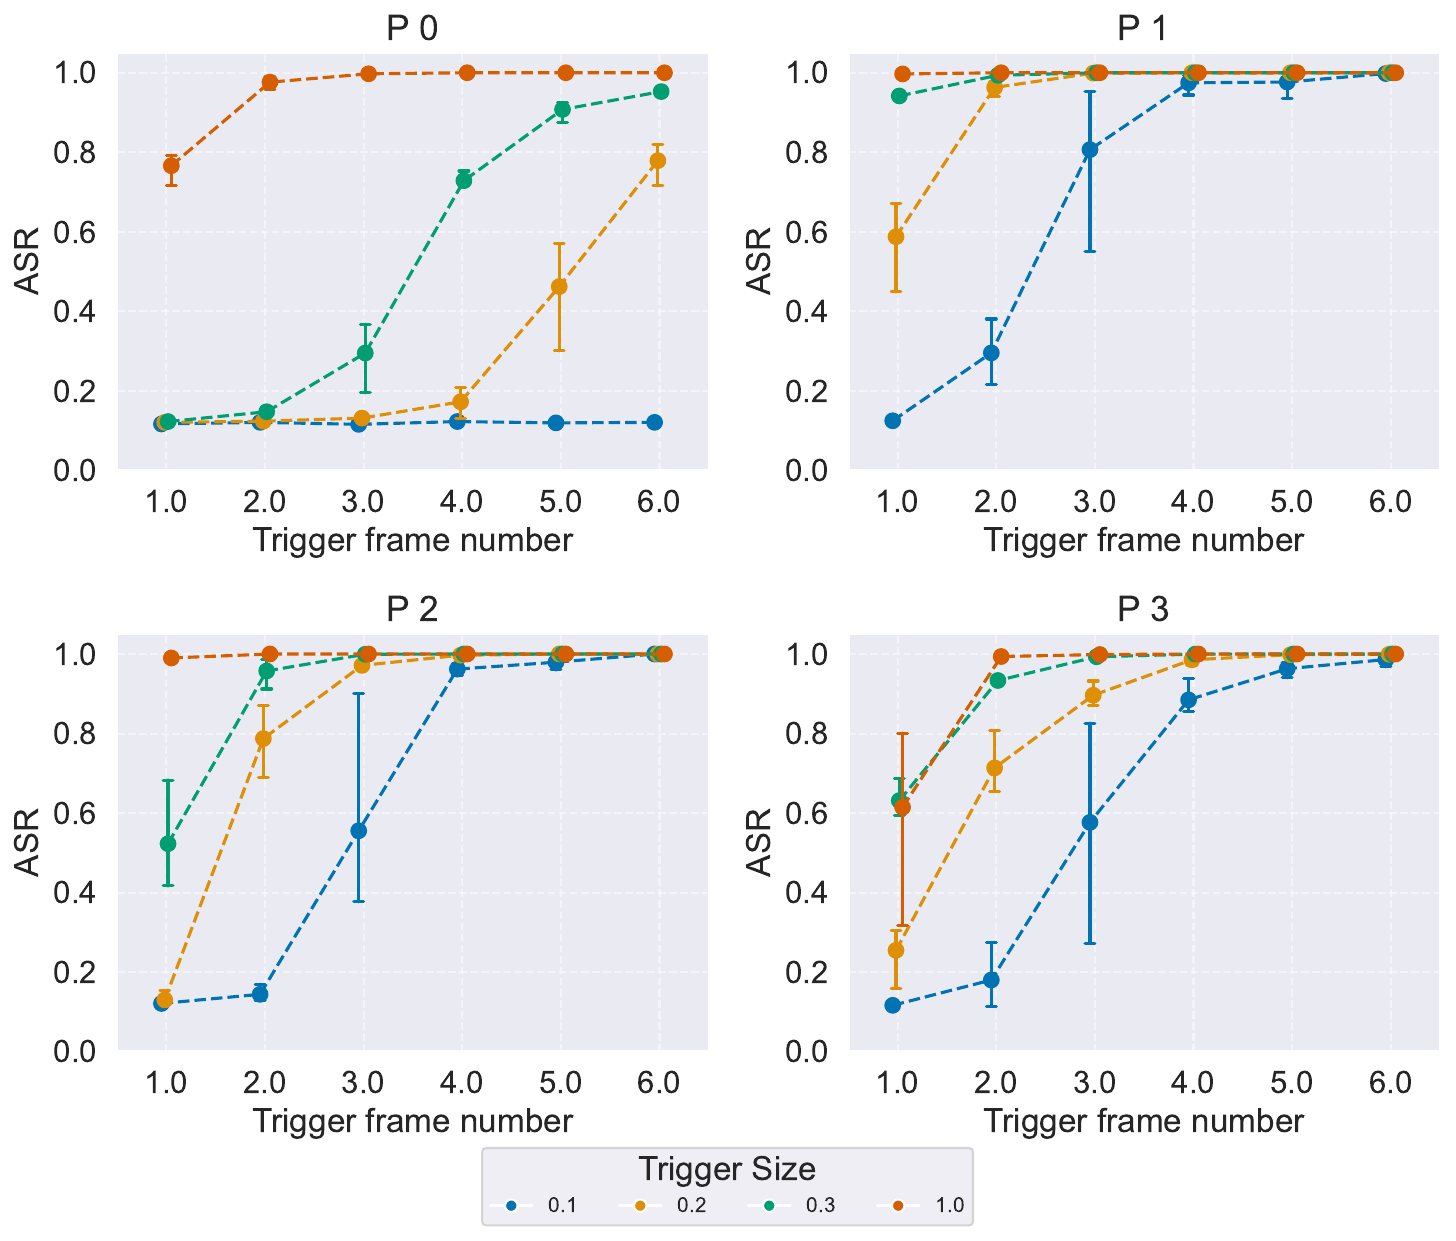}
    %     \caption{ASR Mid position}
    % \end{subfigure}
    % \hfill
    % % \begin{subfigure}[b]{0.49\linewidth}
    % %     \includegraphics[width=\linewidth]{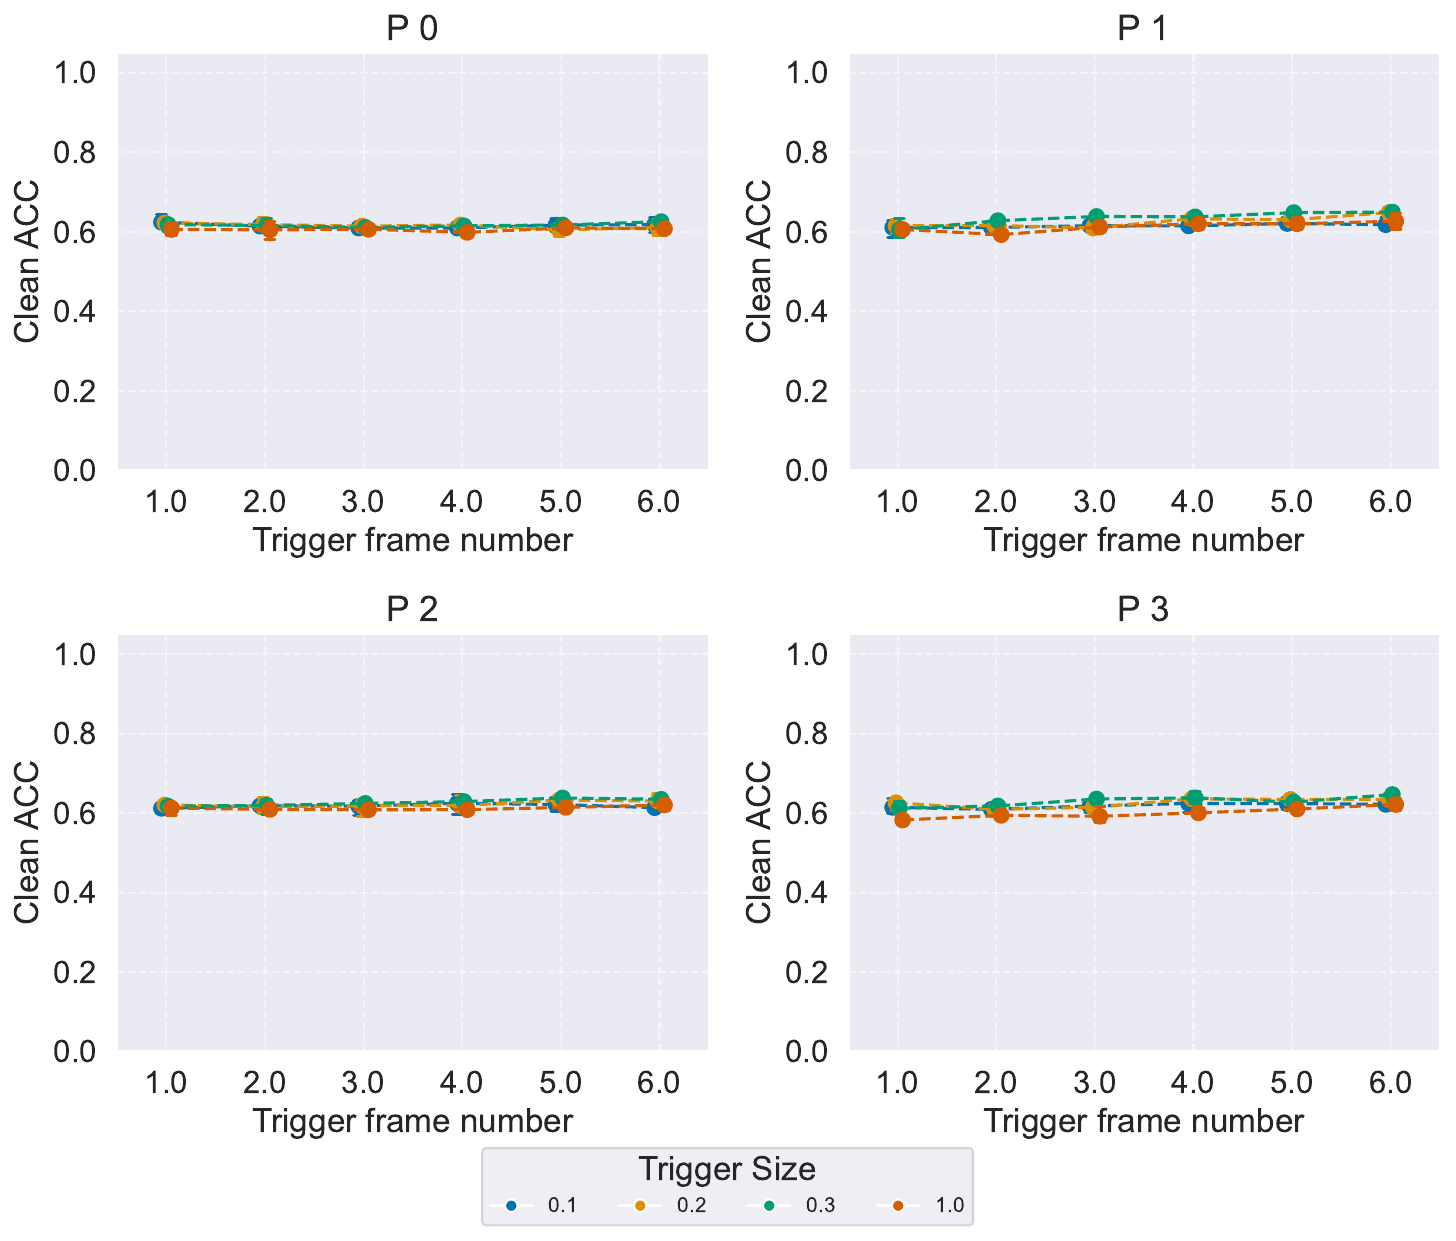}
    % %     \caption{Clean ACC Mid Position}
    % % \end{subfigure}
    % \begin{subfigure}[b]{0.49\linewidth}
    %     \includegraphics[width=\linewidth]{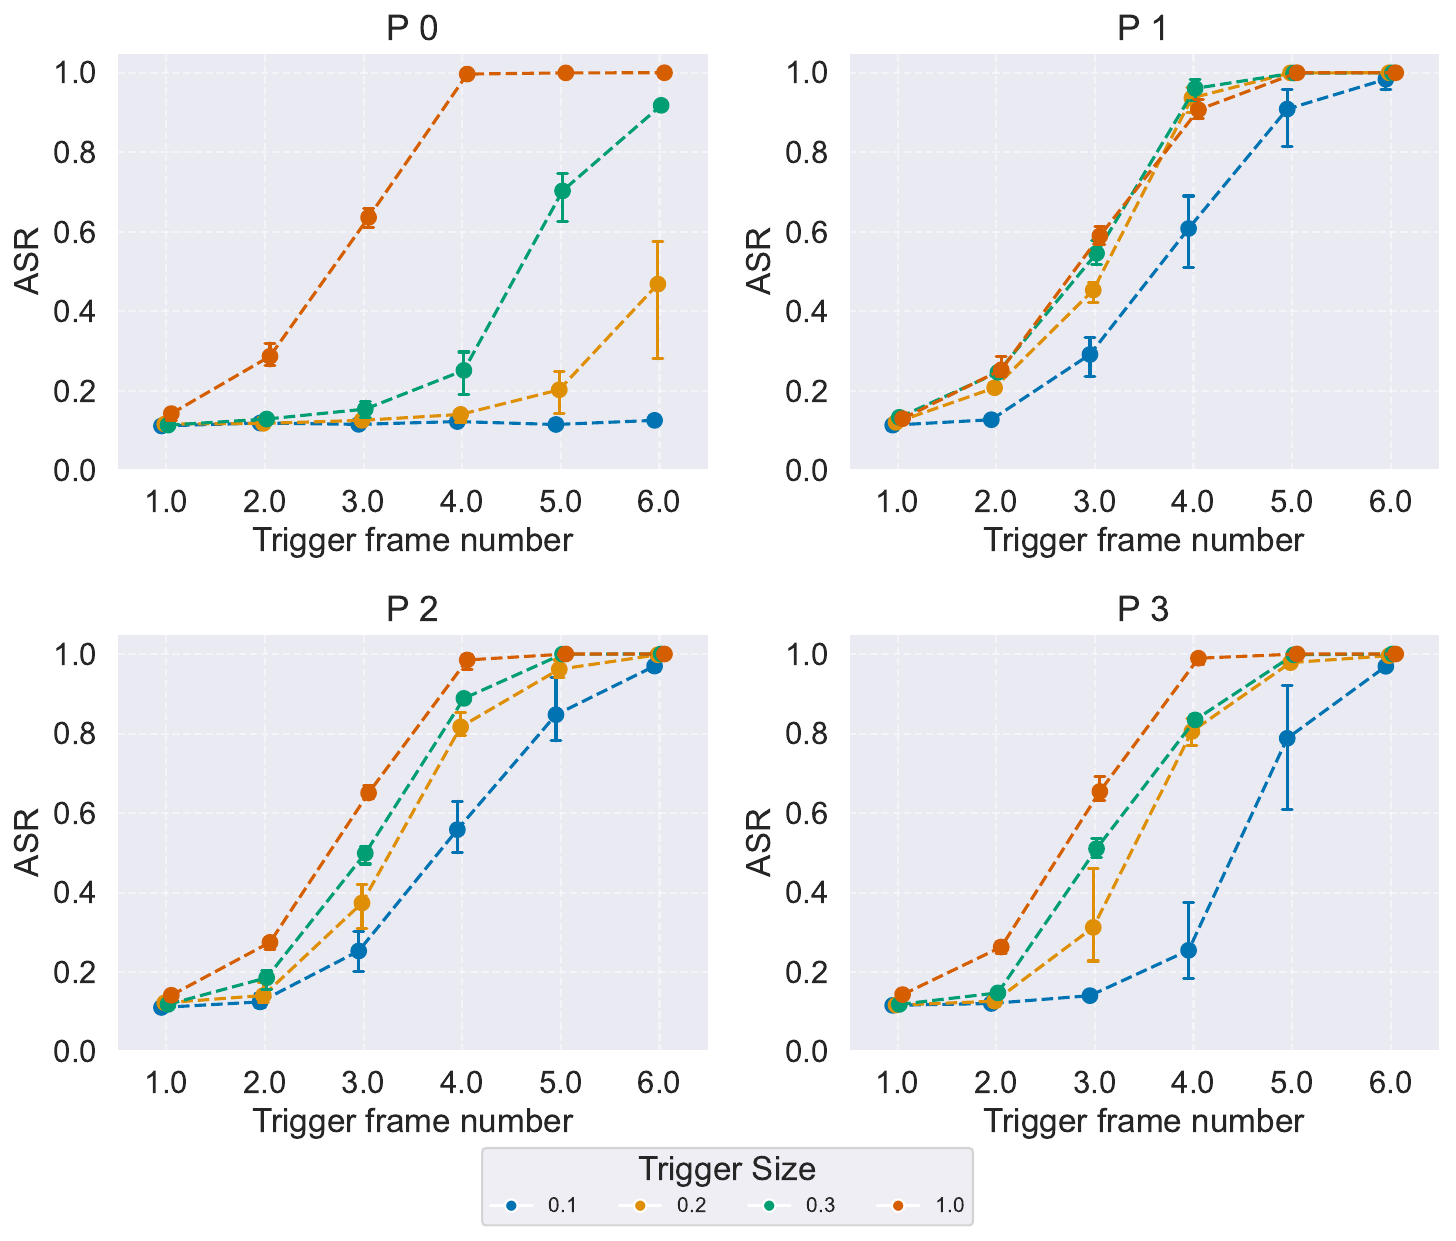}
    %     \caption{ASR End position}
    % \end{subfigure}
    % % \hfill
    % % \begin{subfigure}[b]{0.49\linewidth}
    % %     \includegraphics[width=\linewidth]{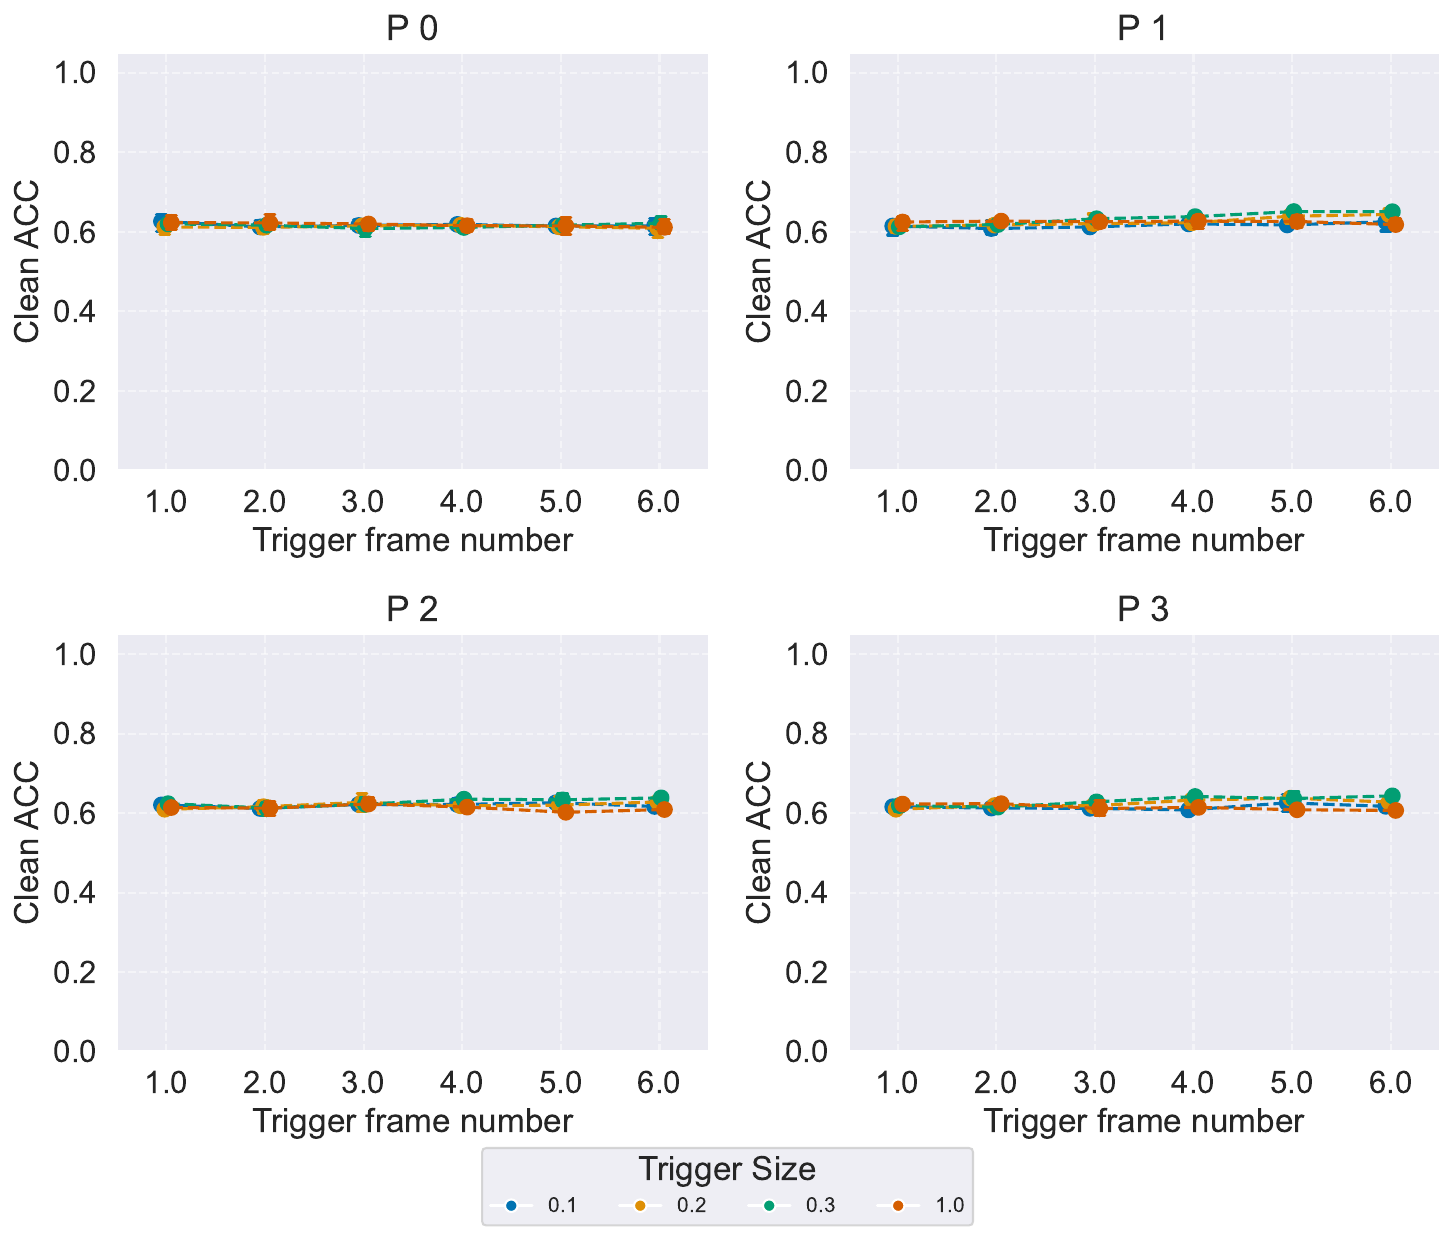}
    % %     \caption{Clean ACC End Position}
    % % \end{subfigure}
    
    \caption{All graphs containing ASR and Clean accuracy for the cifar10-DVS dataset with strobing triggers with a single frame of clean gap.}
    \label{fig:cifar_graphs_strobe}
\end{figure*}

% \begin{figure*}[!ht]
%     \centering

%     \begin{subfigure}[b]{0.49\linewidth}
%         \includegraphics[width=\linewidth]{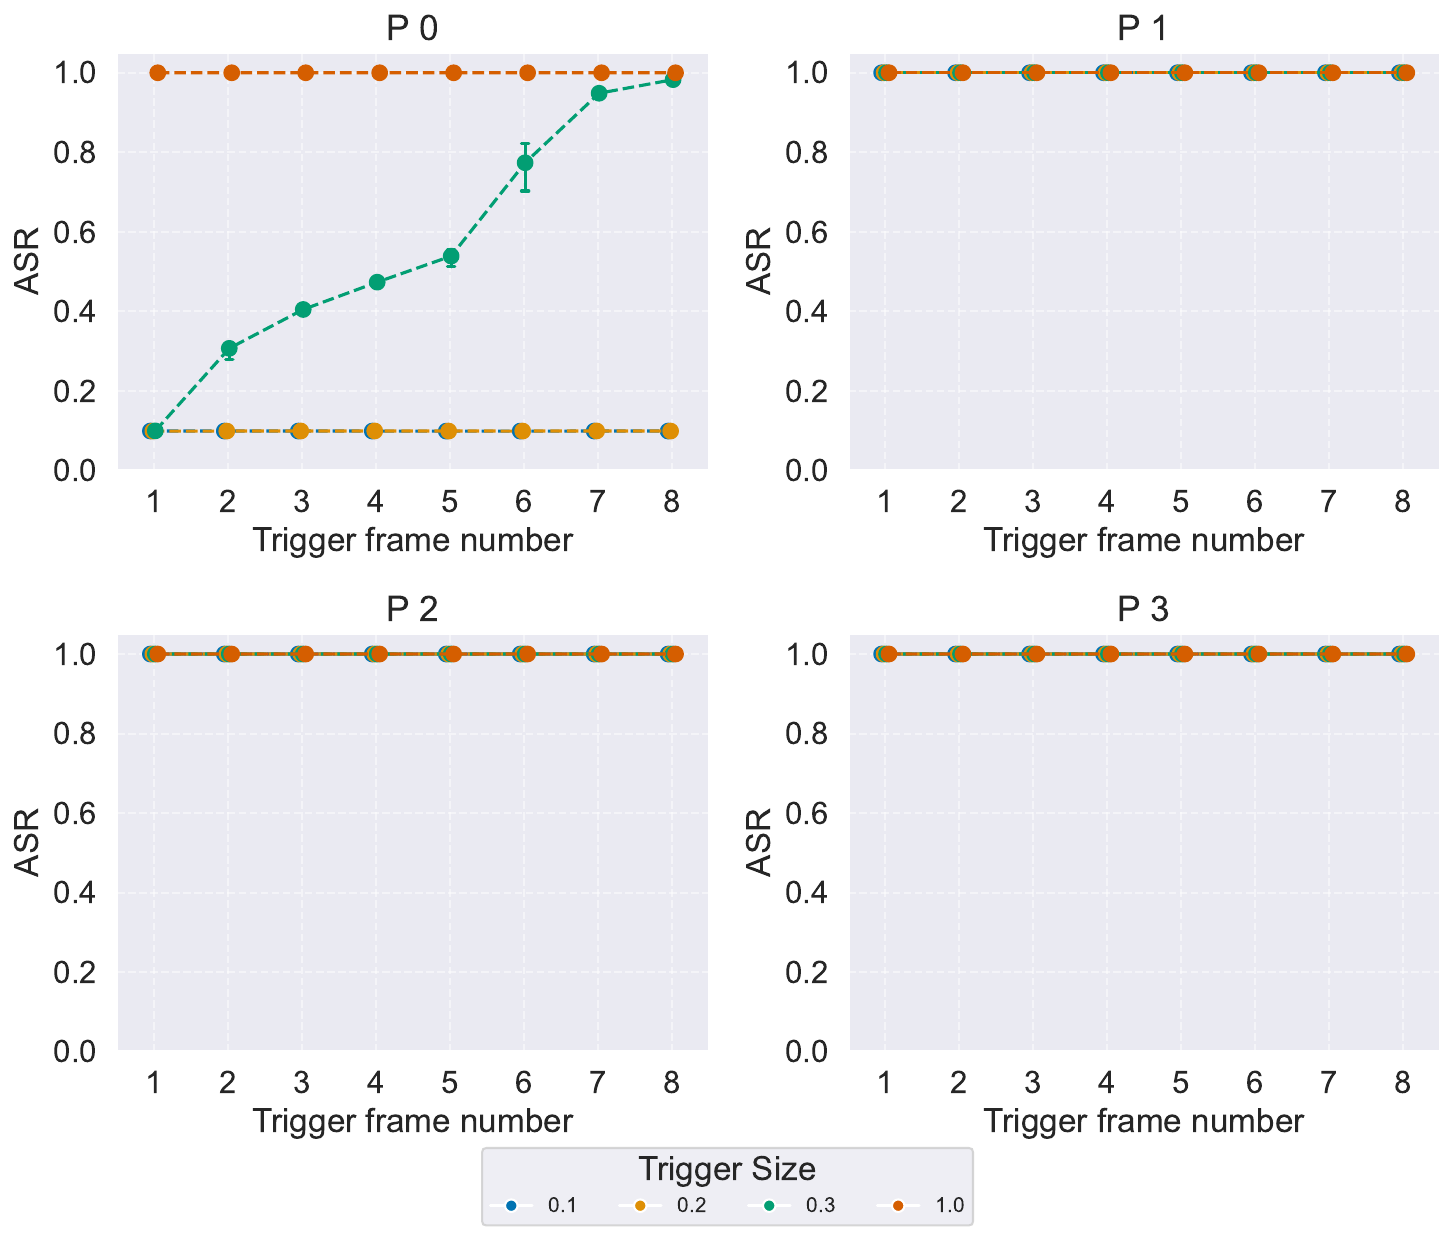}
%         \caption{ASR Start position}
%     \end{subfigure}
%     \hfill
%     \begin{subfigure}[b]{0.49\linewidth}
%         \includegraphics[width=\linewidth]{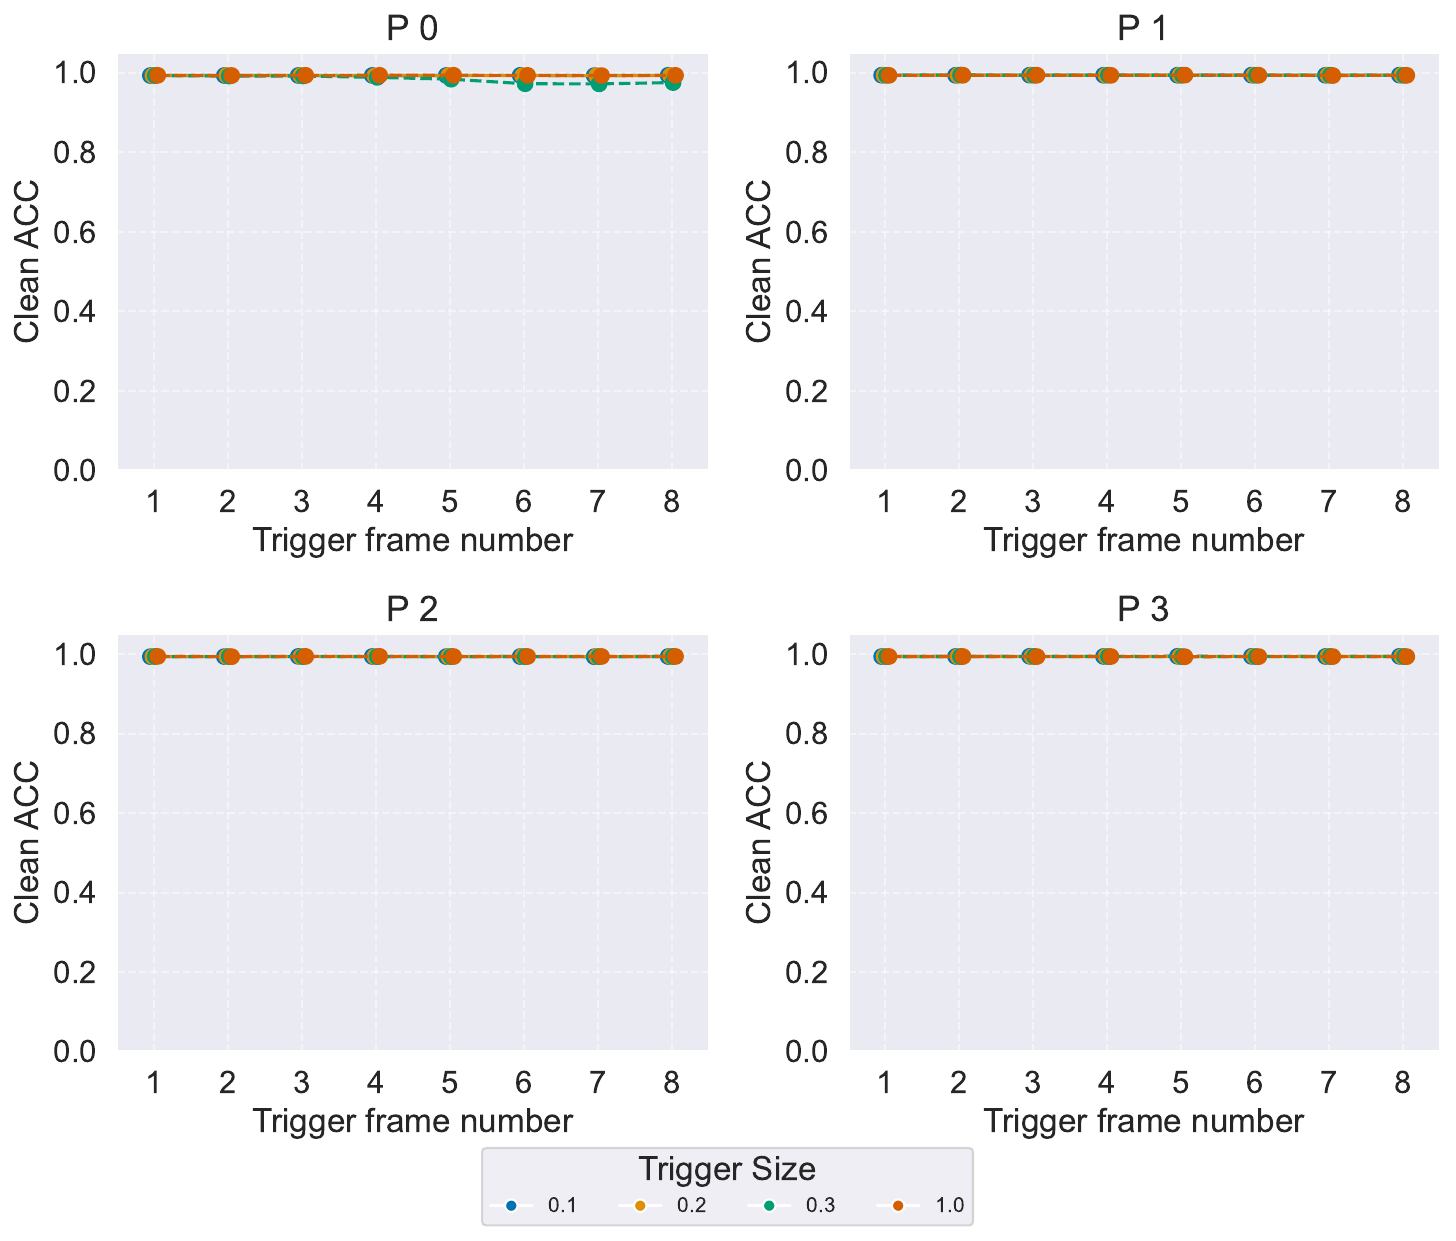}
%         \caption{Clean ACC Start Position}
%     \end{subfigure}
    
%     \begin{subfigure}[b]{0.49\linewidth}
%         \includegraphics[width=\linewidth]{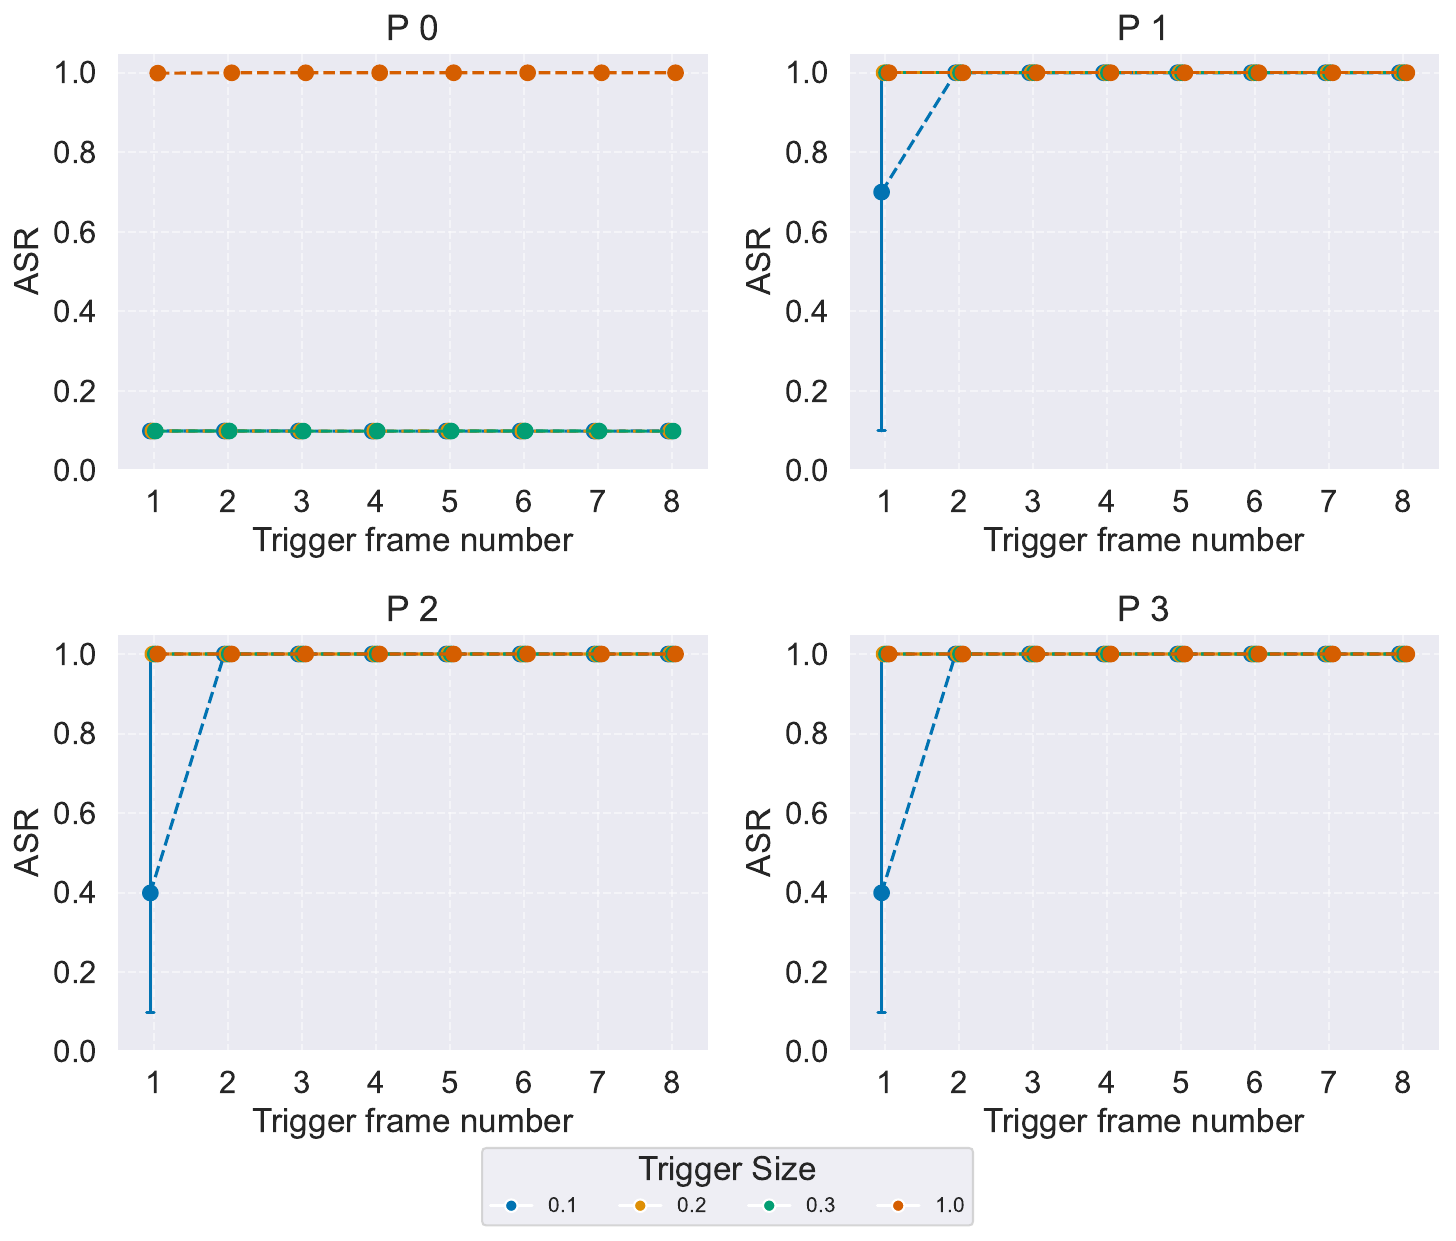}
%         \caption{ASR Mid position}
%     \end{subfigure}
%     \hfill
%     \begin{subfigure}[b]{0.49\linewidth}
%         \includegraphics[width=\linewidth]{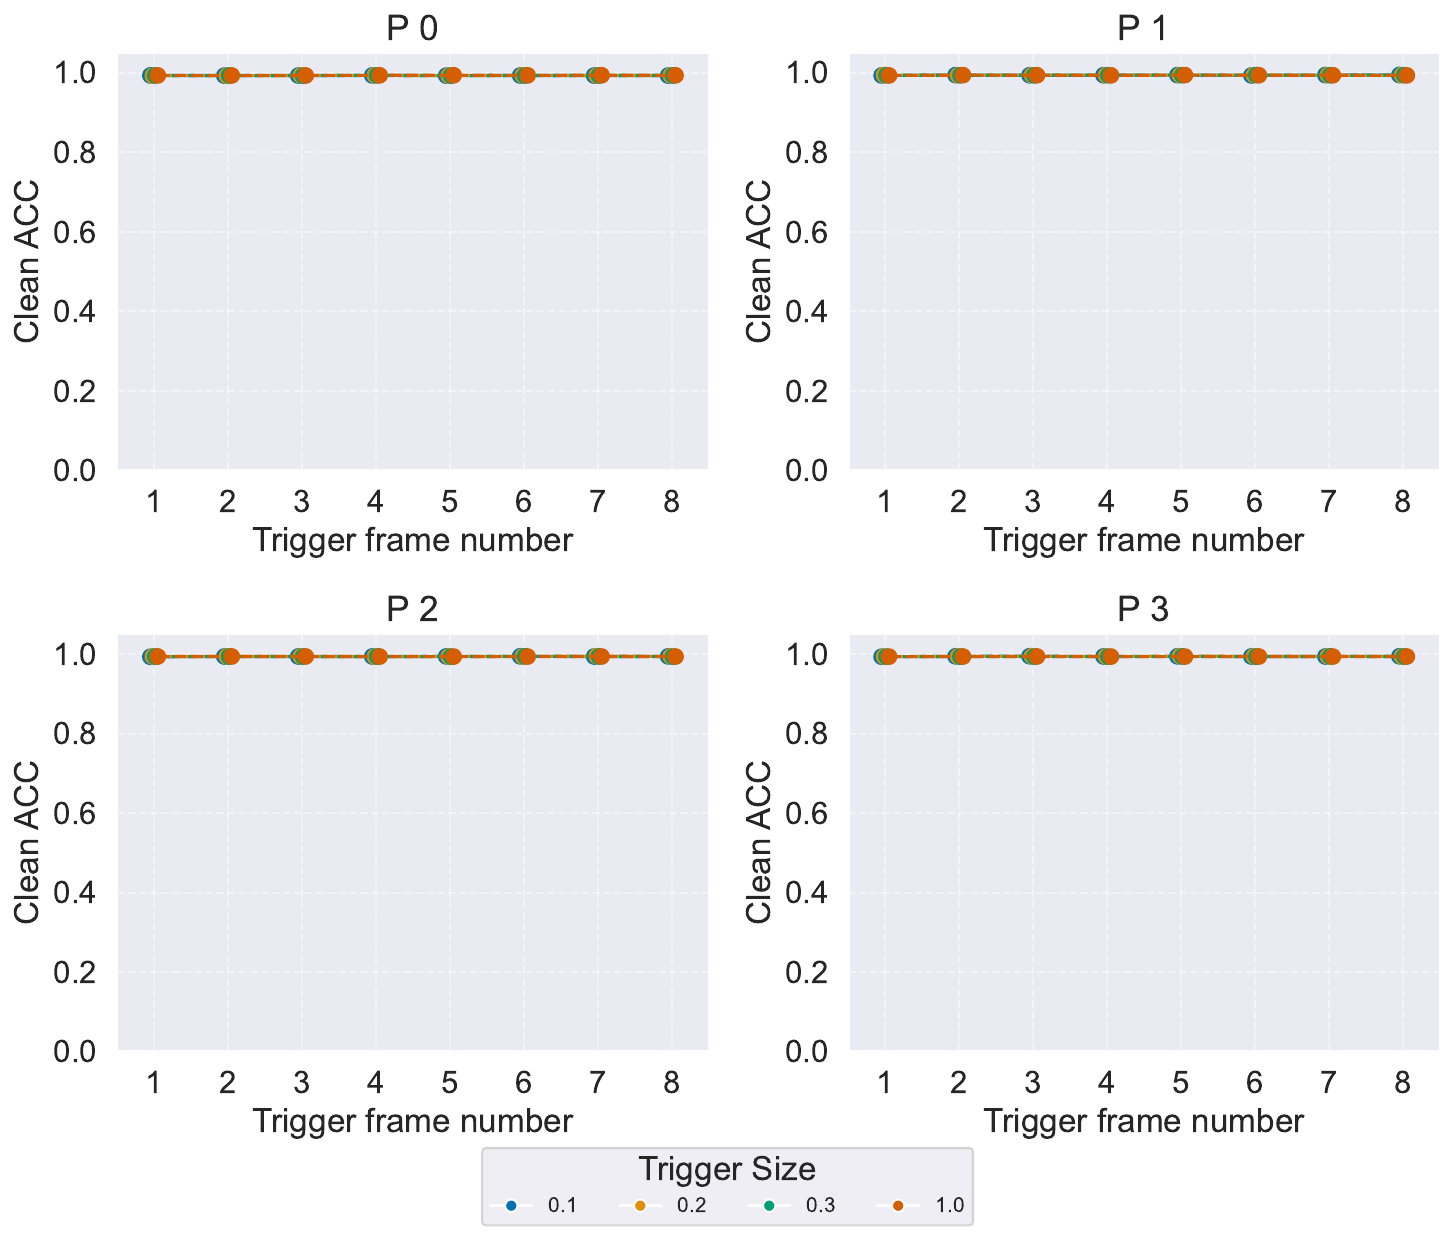}
%         \caption{Clean ACC Mid Position}
%     \end{subfigure}

%     \begin{subfigure}[b]{0.49\linewidth}
%         \includegraphics[width=\linewidth]{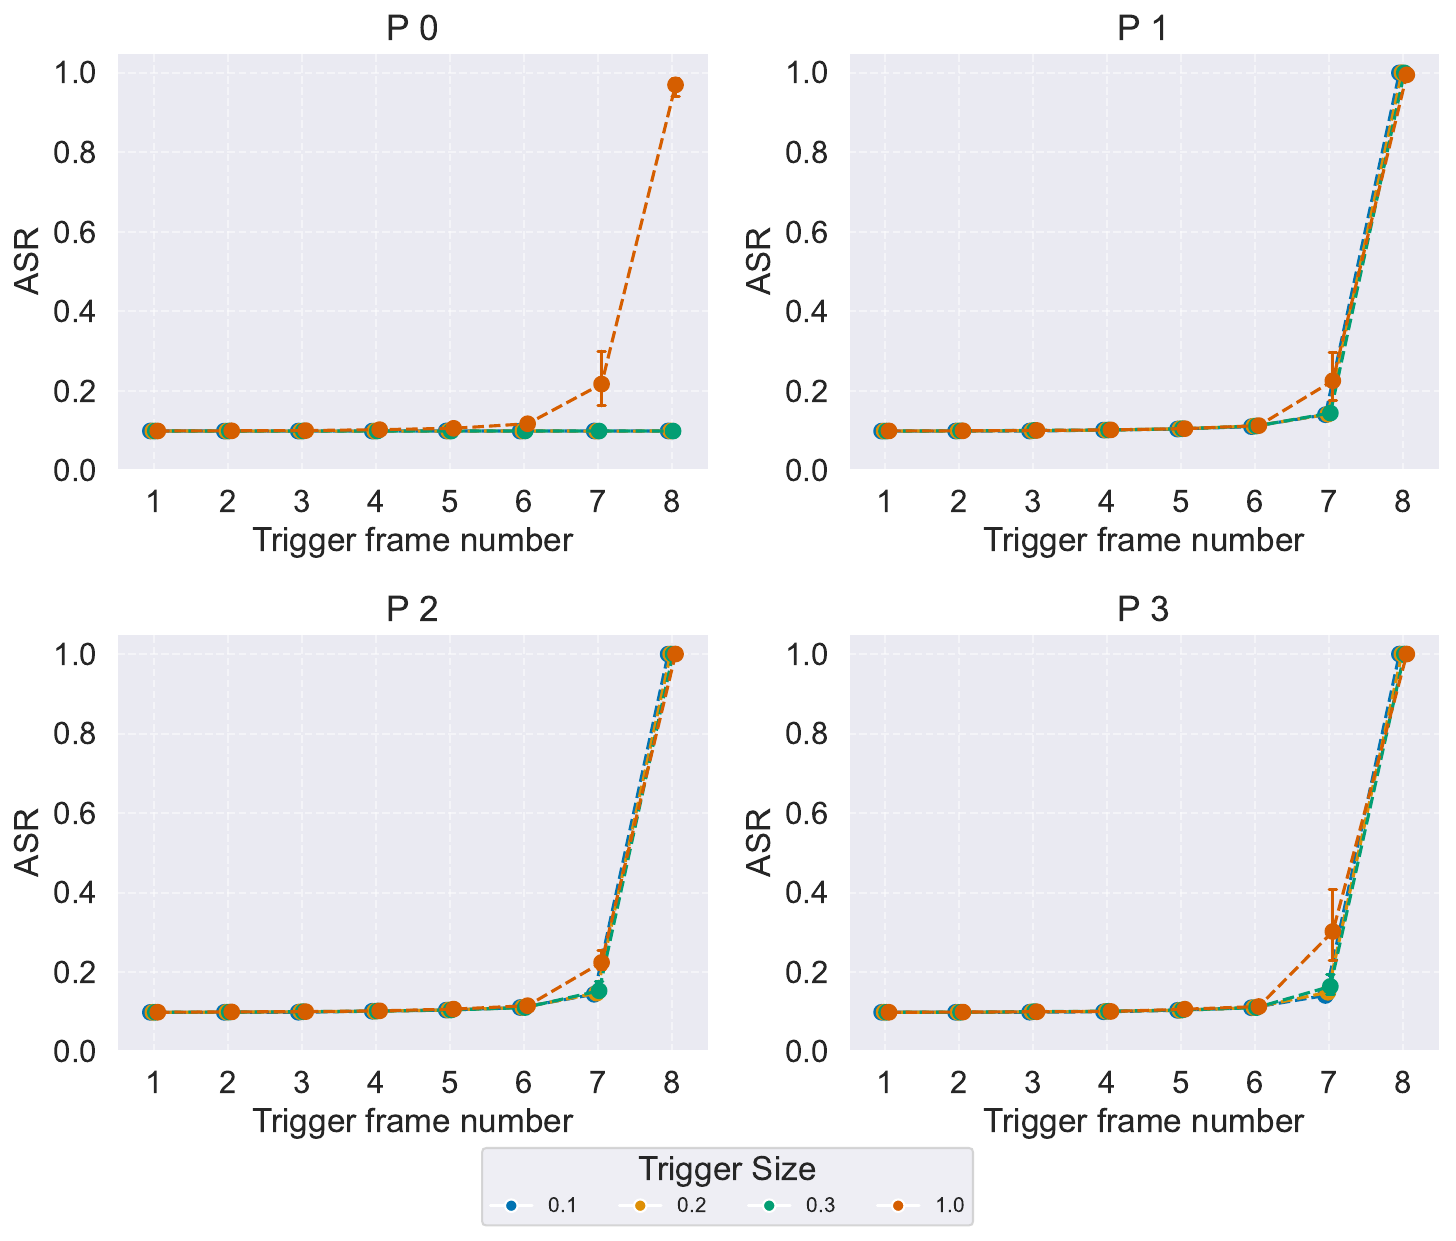}
%         \caption{ASR End position}
%     \end{subfigure}
%     \hfill
%     \begin{subfigure}[b]{0.49\linewidth}
%         \includegraphics[width=\linewidth]{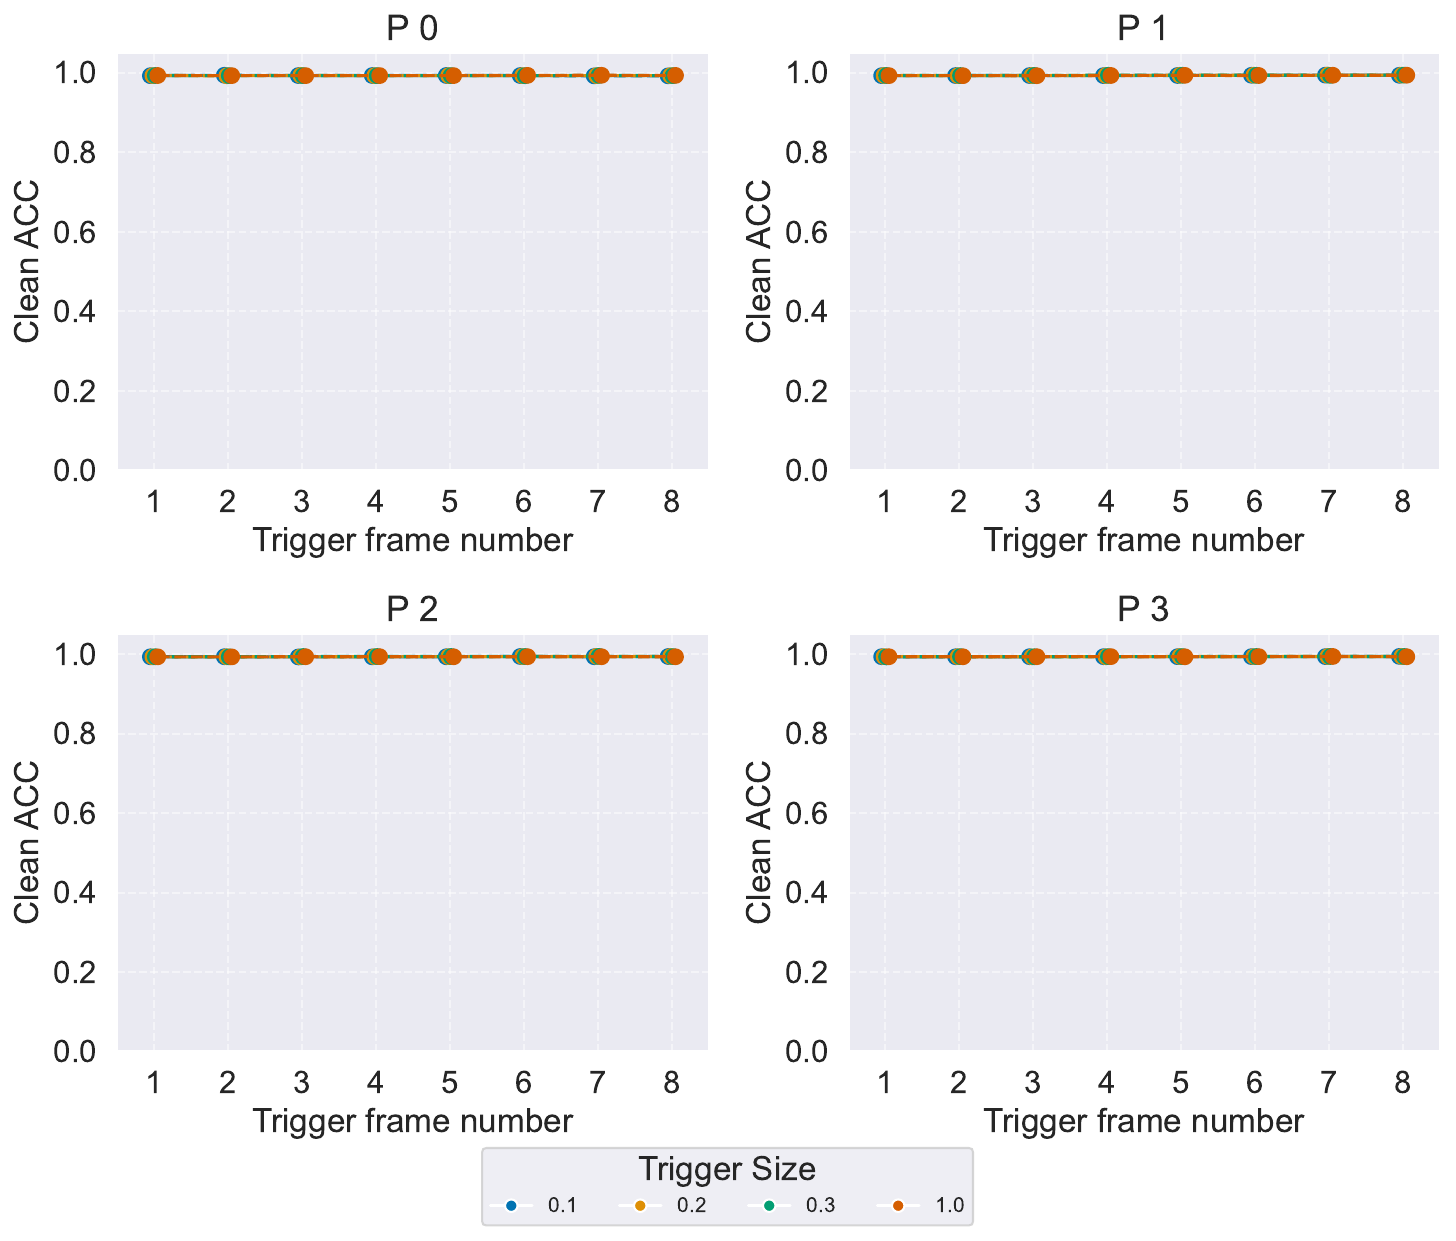}
%         \caption{Clean ACC End Position}
%     \end{subfigure}
    
%     \caption{All graphs containing ASR and Clean accuracy for the NMNIST dataset with continuous triggers.}
%     \label{fig:mnist_graphs}
% \end{figure*}

\begin{figure*}[!ht]
    \centering

    \begin{subfigure}[b]{0.49\linewidth}
        \includegraphics[width=\linewidth]{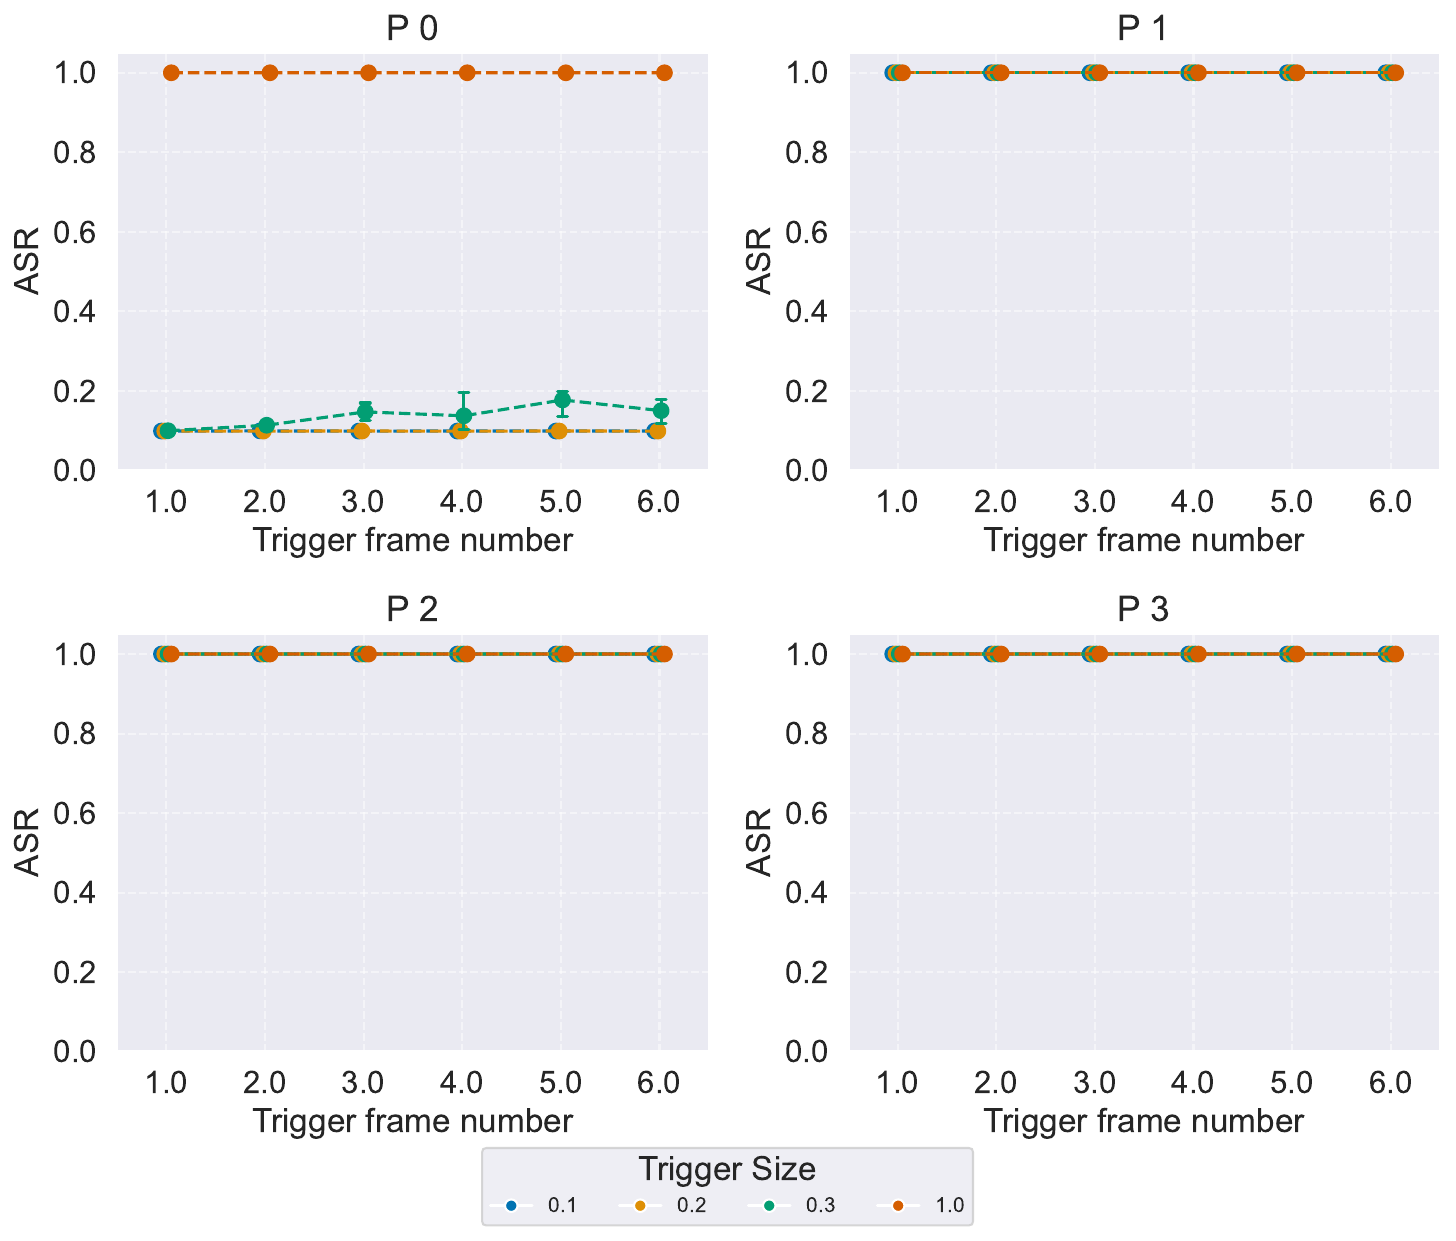}
        \caption{ASR Start position}
    \end{subfigure}
    \hfill
    \begin{subfigure}[b]{0.49\linewidth}
        \includegraphics[width=\linewidth]{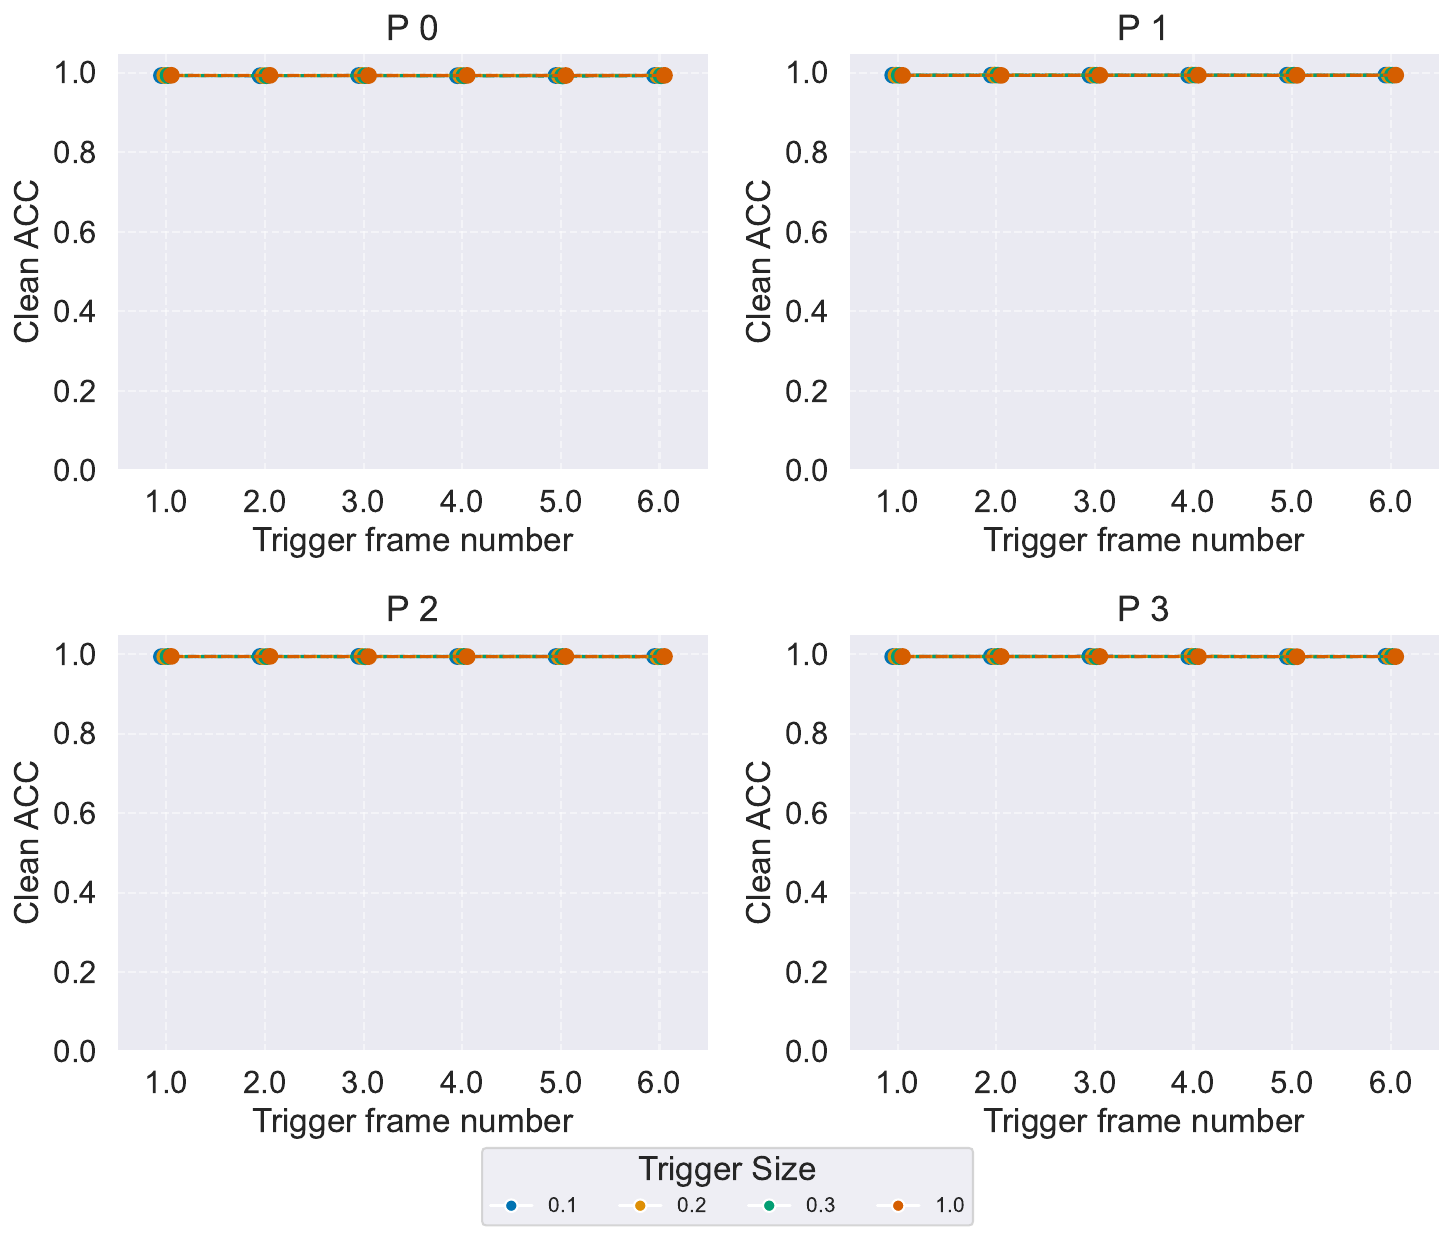}
        \caption{Clean ACC Start Position}
    \end{subfigure}
    
    % \begin{subfigure}[b]{0.49\linewidth}
    %     \includegraphics[width=\linewidth]{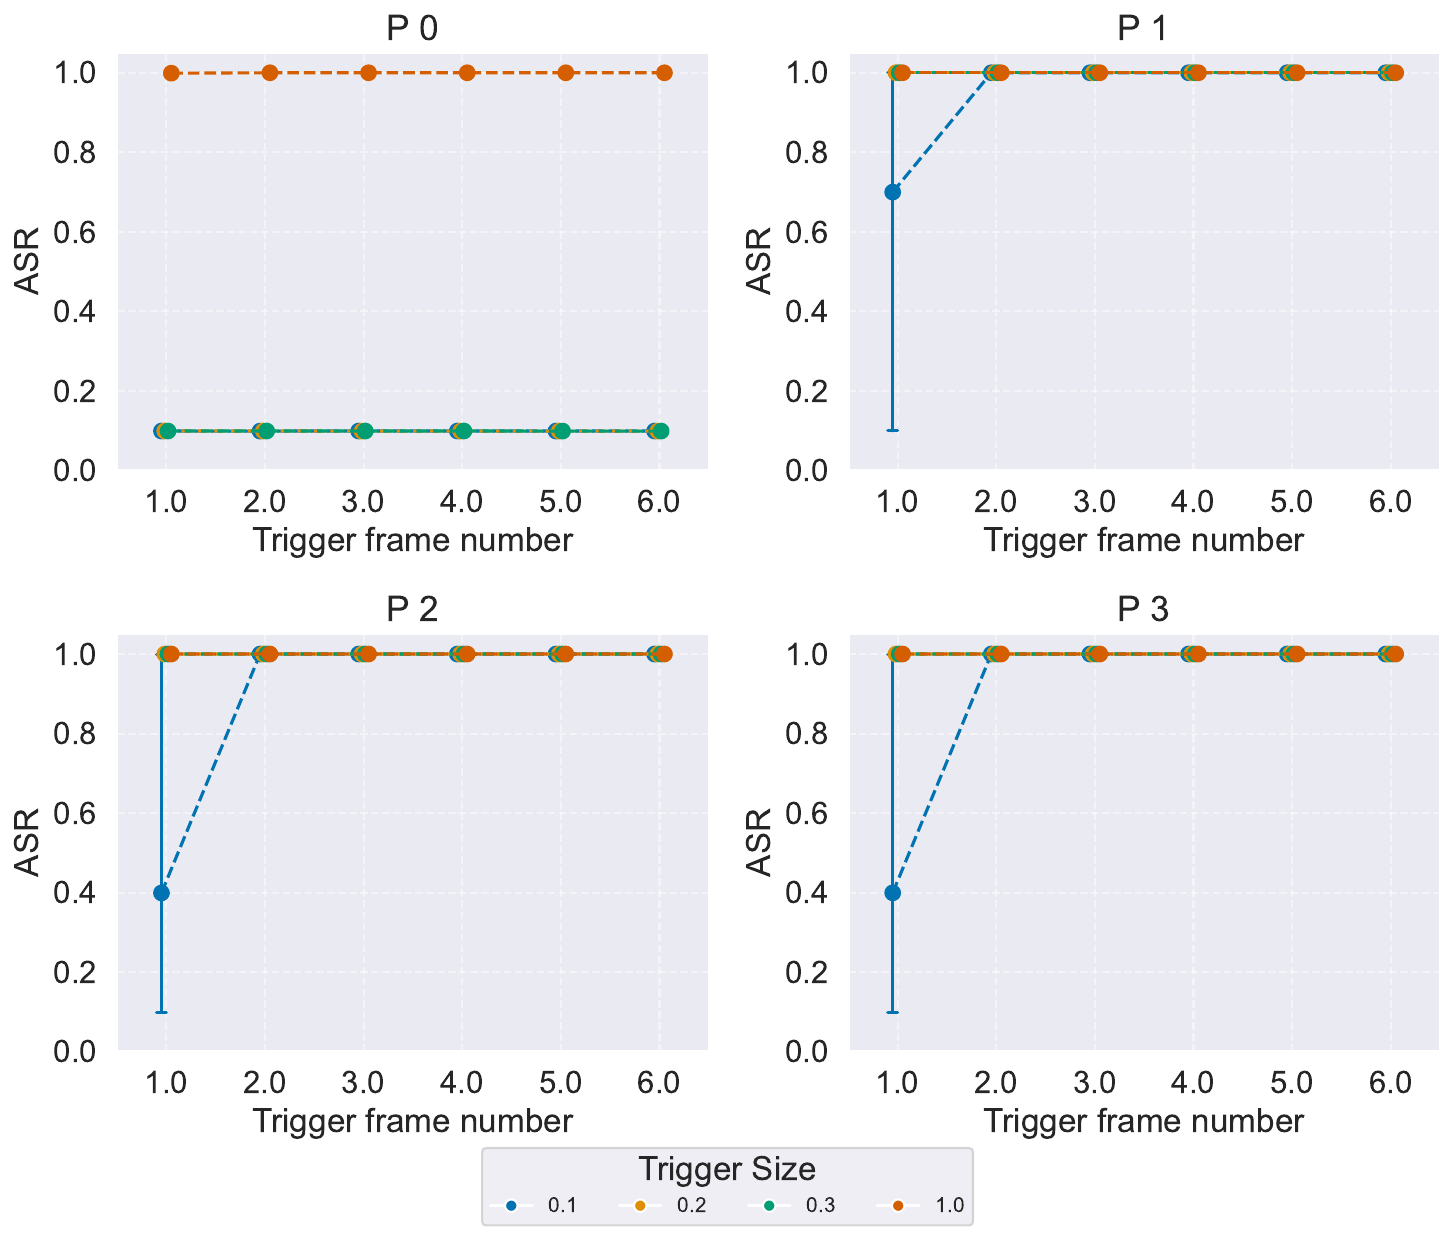}
    %     \caption{ASR Mid position}
    % \end{subfigure}
    % \hfill
    % % \begin{subfigure}[b]{0.49\linewidth}
    % %     \includegraphics[width=\linewidth]{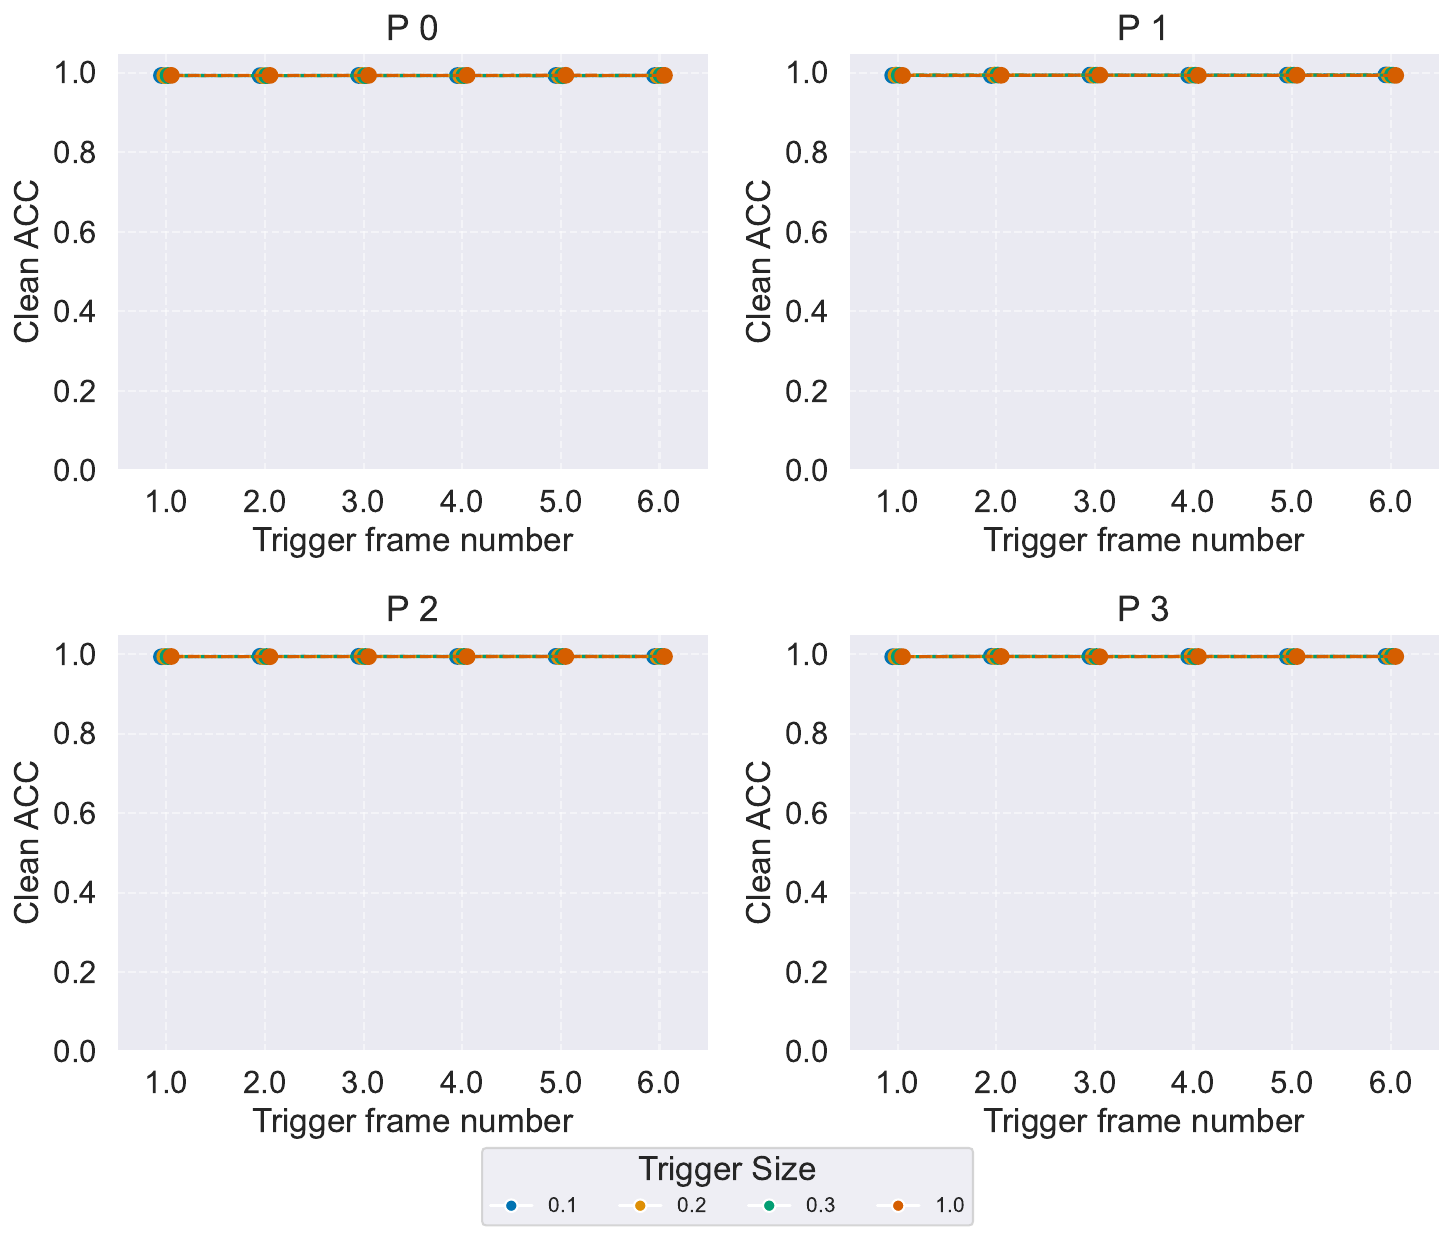}
    % %     \caption{Clean ACC Mid Position}
    % % \end{subfigure}
    % \begin{subfigure}[b]{0.49\linewidth}
    %     \includegraphics[width=\linewidth]{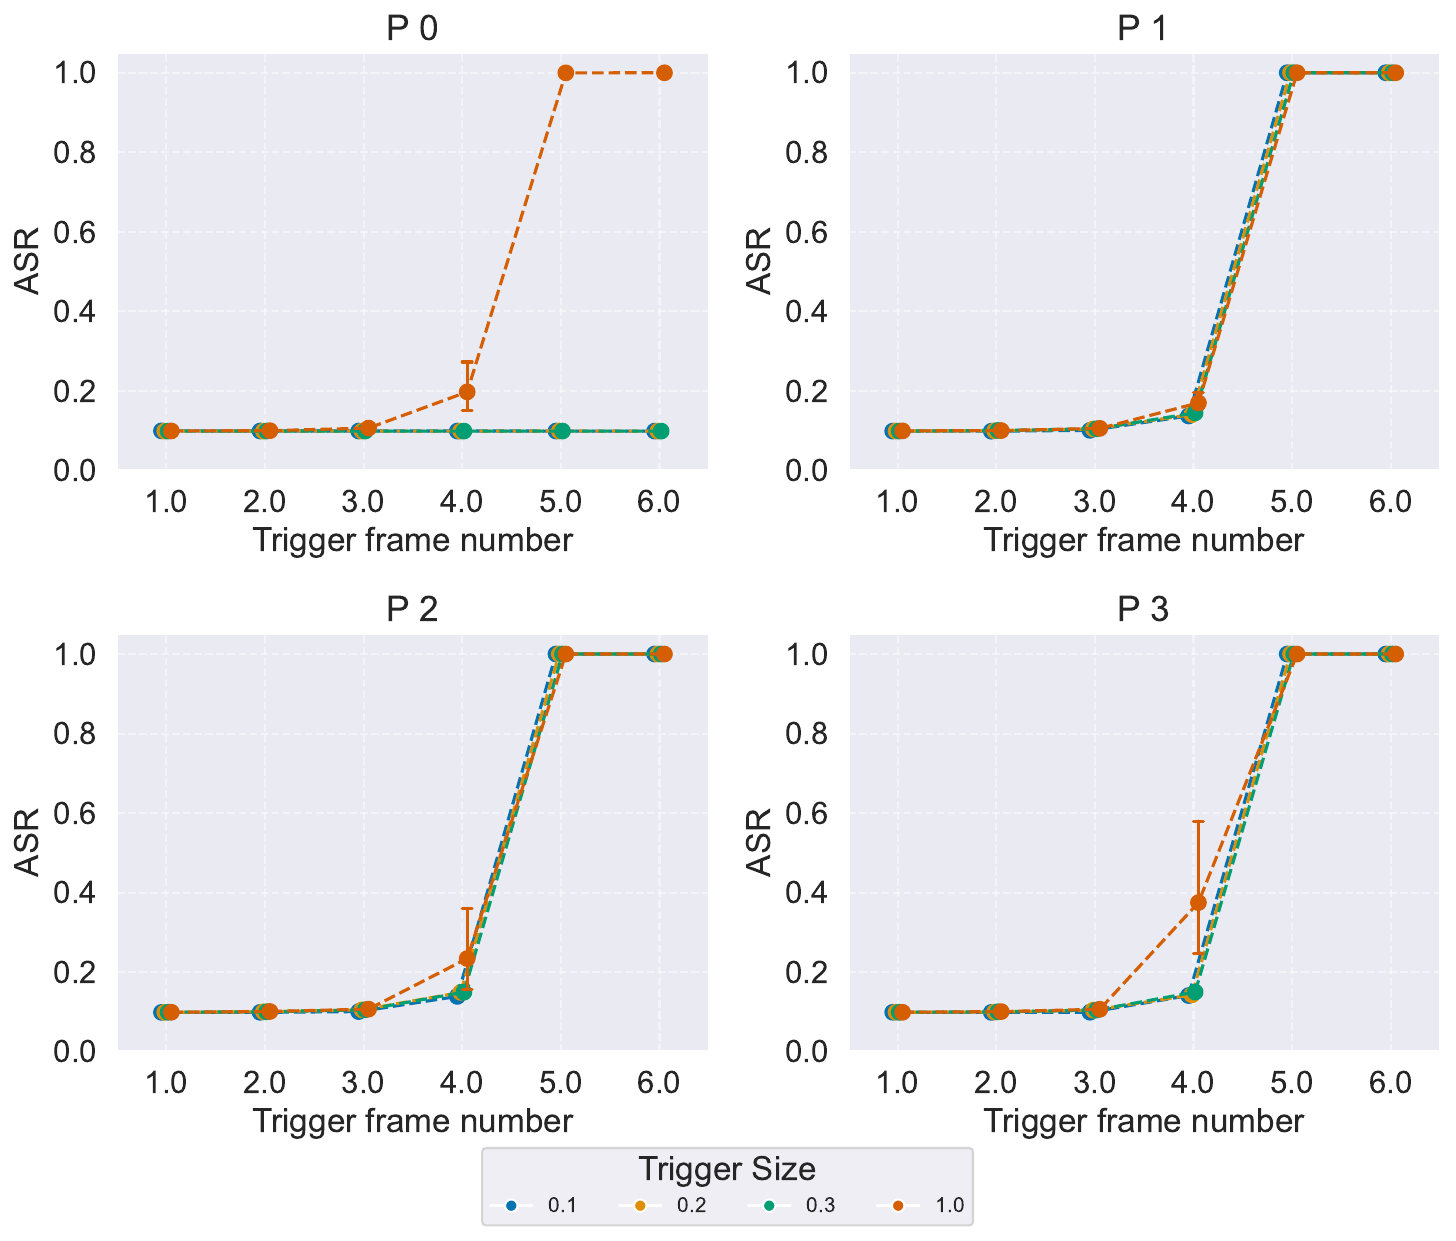}
    %     \caption{ASR End position}
    % \end{subfigure}
    % % \hfill
    % % \begin{subfigure}[b]{0.49\linewidth}
    % %     \includegraphics[width=\linewidth]{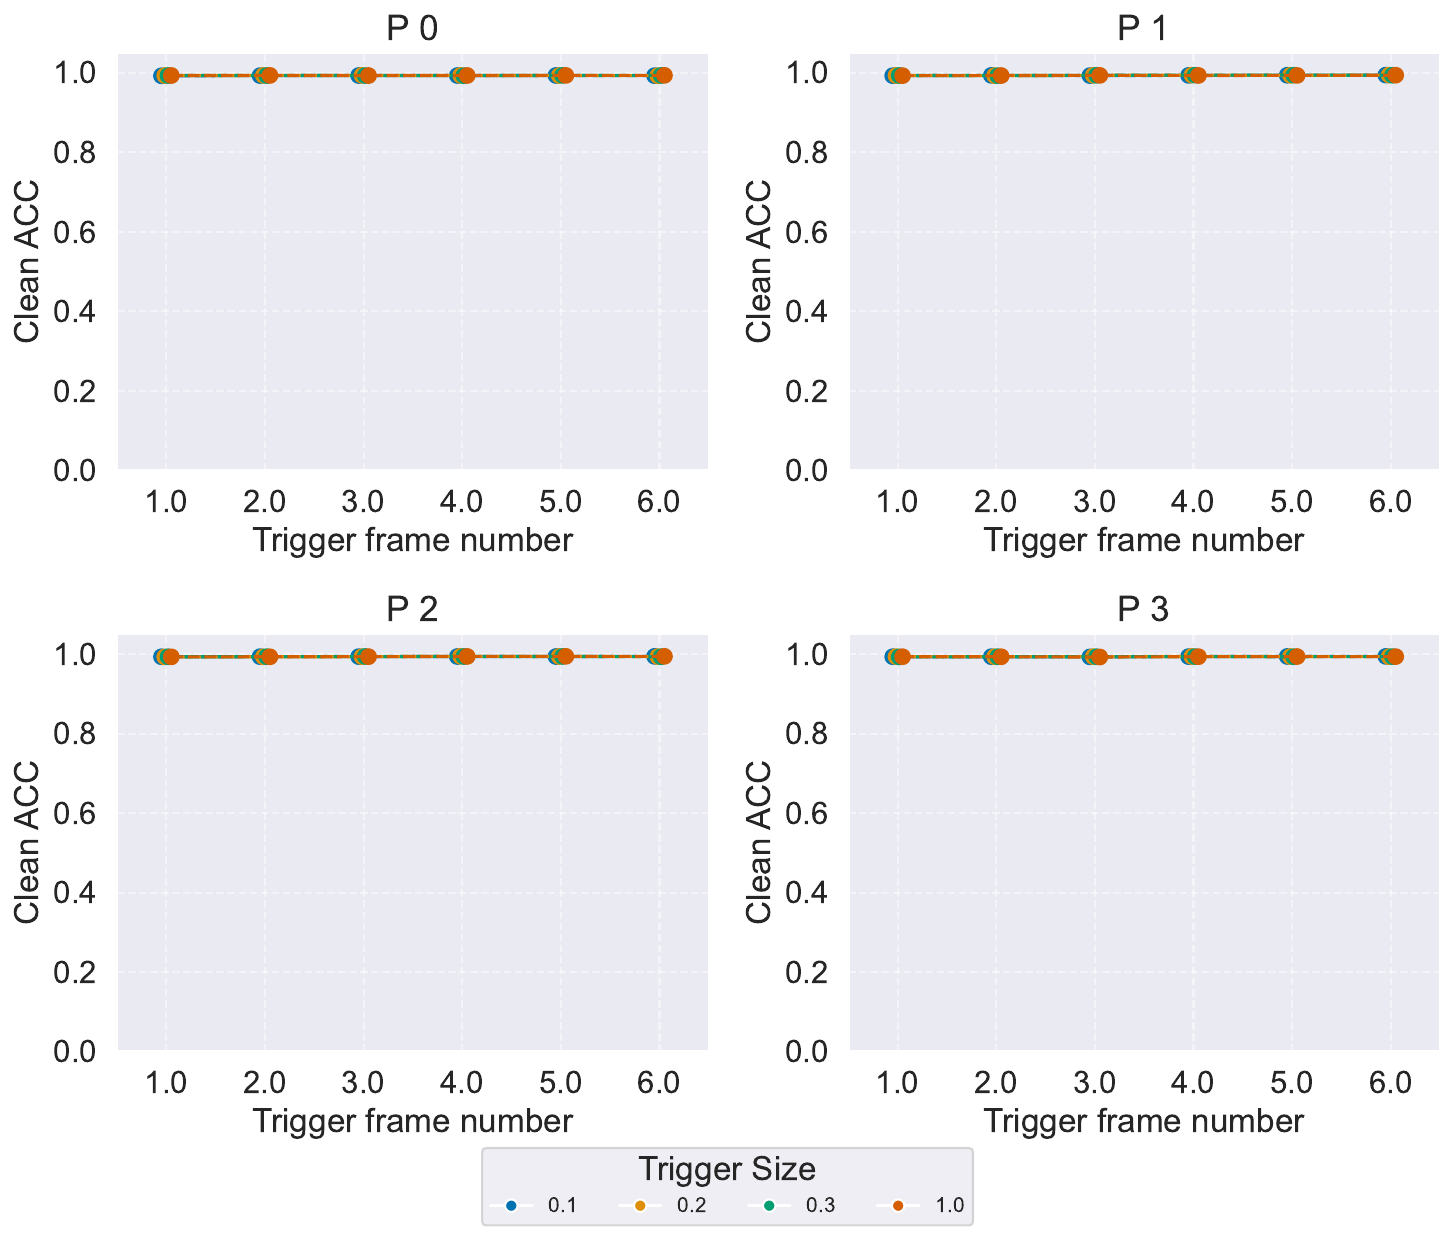}
    % %     \caption{Clean ACC End Position}
    % % \end{subfigure}
    
    \caption{All graphs containing ASR and Clean accuracy for the NMNIST dataset with strobing triggers with a single frame of clean gap.}
    \label{fig:mnist_graphs_strobe}
\end{figure*}
